# Supplementary material for: Quantum State and Process Tomography of Energy Transfer Systems via Ultrafast Spectroscopy
Source: arXiv:1006.4866 source file (2011-10-28)
Supplement: Supplementary file 1 [file manuscript2_revised_092911_supplementary.pdf]

# Quantum State and Process Tomography of Energy Transfer Systems via Ultrafast Spectroscopy

Joel Yuen-Zhou, Jacob J. Krich, Masoud Mohseni, and Alán Aspuru-Guzik\*

*Department of Chemistry and Chemical Biology,*

*Harvard University, Cambridge, MA 02138*

## Abstract

The description of excited state dynamics in energy transfer systems constitutes a theoretical and experimental challenge in modern chemical physics. An experimental protocol which systematically characterizes both coherent and dissipative processes at the level of the evolving quantum state of the probed chromophores is desired. Here, we show that a set of two-color photon-echo experiments performs quantum state tomography (QST) of the one-exciton manifold of a dimer by reconstructing its density matrix in real time. This possibility in turn allows for a complete description of excited state dynamics via quantum process tomography (QPT). Simulations of a noisy QPT experiment for an inhomogeneously broadened ensemble of model excitonic dimers show that the protocol distills rich information about coherent and dissipative excitonic dynamics, which appear nontrivially hidden in the signal monitored in single realizations of four-wave mixing experiments. Our study represents a novel method for analyzing the content of nonlinear optical experiments utilizing concepts and tools from quantum information processing (QIP), and opens interesting possibilities for understanding, control, and manipulation of excitonic systems.

---

\*Electronic address: [aspuru@chemistry.harvard.edu](mailto:aspuru@chemistry.harvard.edu)

Excitonic systems and the processes triggered upon their interaction with electromagnetic radiation are of fundamental physical and chemical interest . In nonlinear optical spectroscopy (NLOS), a series of ultrafast femtosecond pulses induces coherent vibrational and electronic dynamics in a molecule or nanomaterial, and the nonlinear polarization of the excitonic system is monitored both in the time and frequency domains . To interpret these experiments, theoretical modeling has proven essential, framed within the Liouville space formalism popularized by Mukamel . Implicit in these calculations is the evolution of the quantum state of the dissipative system in the form of a density matrix. The detected polarization contains information of the time dependent density matrix of the system, although not in the most transparent way. An important problem is whether these experiments allow quantum state tomography (QST), that is, the determination of the density matrix of the probed system at different instants of time. A more ambitious question is if a complete characterization of the quantum dynamics of the system can be performed via quantum process tomography (QPT) , a protocol that we define in the next section. In this article, we show that both QST and QPT are possible for the single-exciton manifold of a coupled dimer of chromophores with a series of two-color photon echo (PE) experiments. We also present numerical simulations on a model system and show that robust QST and QPT is achievable even in the presence of experimental noise as well as inhomogeneous broadening. The present work offers an intriguing perspective on the amount of quantum information accessible through nonlinear optical spectroscopy, and hence opens interesting avenues for spectroscopy of energy transfer systems via a Quantum Information Processing (QIP) approach.

This article provides a conceptual presentation, and interested readers may find derivations and technical details in the Supporting Information (SI).

### Basic concepts of QPT

Consider a quantum system which interacts with an environment. We can describe the full state of the system and the environment at time  $T$  by the density matrix  $\rho_{\text{total}}(T)$  and the reduced density matrix of the system as  $\rho(T) = \text{Tr}_B \rho_{\text{total}}(T)$ , where the trace is over the degrees of freedom of the environment (also called the bath). If the initial state is a product,  $\rho_{\text{total}}(0) = \rho(0) \otimes \rho_B$  (always with the same bath state  $\rho_B$ ), then the evolution of the system may be expressed as a linear transformation :

$$\rho_{ab}(T) = \sum_{cd} \chi_{abcd}(T) \rho_{cd}(0). \quad (1)$$

The central object of this article is the *process matrix*  $\chi(T)$ , which is independent of the initial state  $\rho(0)$ . As opposed to master equations which are written in differential form, Eq. 1 can be regarded as an integrated equation of motion for every  $T$ . It holds both for Markovian and non-Markovian dynamics of the bath. Note that  $\chi(T)$  completely characterizes the dynamics of the system. Preserving Hermiticity, trace, and positivity of  $\rho(T)$  imply, respectively, the following relations (SI-I),

$$\chi_{abcd}(T) = \chi_{badc}^*(T), \quad (2)$$

$$\sum_a \chi_{aacd}(T) = \delta_{cd}, \quad (3)$$

$$\sum_{abcd} z_{ac}^* \chi_{abcd}(T) z_{bd} \geq 0, \quad (4)$$

where  $z$  is any complex valued vector. Using Eqs. 2 and 3, for a system in a  $d$ -dimensional Hilbert space,  $\chi(T)$  is determined by  $d^4 - d^2$  real valued parameters. Operationally, QPT can be defined as an experimental protocol to obtain  $\chi(T)$ . Spectroscopically,  $\chi(T)$  may be reconstructed by measuring  $\rho(T)$  (i.e., performing QST) given some choice of initial state  $\rho(0)$ , where the  $\rho(0)$  are chosen successively from a complete set of initial states. Since we are interested in energy transfer dynamics, this procedure shall be performed at several values of  $T$ . In this article, we show how to perform QPT for a model coupled excitonic dimer using two-color heterodyne photon-echo experiments.

### Description of the system and its interaction with light

Consider an excitonic dimer interacting with a bath of phonons. The excitonic part of the Hamiltonian, describing the system with the environment frozen in place, is given by :

$$\begin{aligned} H_S &= \omega_A a_A^\dagger a_A + \omega_B a_B^\dagger a_B + J(a_A^\dagger a_B + a_B^\dagger a_A) \\ &= \omega_\alpha c_\alpha^\dagger c_\alpha + \omega_\beta c_\beta^\dagger c_\beta. \end{aligned} \quad (5)$$

where  $a_i^\dagger$  and  $c_j^\dagger$  ( $a_i$  and  $c_j$ ) are creation (annihilation) operators for site  $i \in \{A, B\}$  and delocalized  $j \in \{\alpha, \beta\}$  excitons, respectively.  $\omega_A \neq \omega_B$  are the first and second site energies,  $J \neq 0$  is the Coulombic coupling between the chromophores. We define the average of site energies  $\omega = \frac{1}{2}(\omega_A + \omega_B)$ , difference  $\Delta = \frac{1}{2}(\omega_A - \omega_B)$ , and mixing angle  $\theta = \frac{1}{2} \arctan\left(\frac{J}{\Delta}\right)$ . Then  $c_\alpha = \cos \theta a_A + \sin \theta a_B$ ,  $c_\beta = -\sin \theta a_A + \cos \theta a_B$ ,  $\omega_\alpha = \omega + \Delta \sec 2\theta$ , and  $\omega_\beta = \omega - \Delta \sec 2\theta$ . For convenience, we define the single exciton states  $|\alpha\rangle = c_\alpha^\dagger |g\rangle$ ,  $|\beta\rangle = c_\beta^\dagger |g\rangle$ , where  $|g\rangle$  is the ground state, and the biexcitonic state  $|f\rangle = a_A^\dagger a_B^\dagger |g\rangle = c_\alpha^\dagger c_\beta^\dagger |g\rangle$ . The model Hamiltonian does

not account for exciton-exciton binding or repulsion terms, so the energy level of the biexciton is  $\omega_f = \omega_\alpha + \omega_\beta = \omega_A + \omega_B$ . Denoting  $\omega_{ij} \equiv \omega_i - \omega_j$ , we have  $\omega_{\alpha g} = \omega_{f\beta}$  and  $\omega_{\beta g} = \omega_{f\alpha}$ .

We are interested in the perturbation of the excitonic system  $S$  due to three laser pulses:

$$V(t') = -\lambda \sum_{i=1}^3 \hat{\boldsymbol{\mu}} \cdot \mathbf{e}_i E(t' - t_i) \{e^{i\mathbf{k}_i \cdot \mathbf{r} - i\omega_i(t' - t_i)} + c.c.\} \quad (6)$$

Here,  $\lambda$  is the intensity of the electric field, which is assumed weak.  $\hat{\boldsymbol{\mu}}$  is the dipole operator,  $\mathbf{e}_i, t_i, \mathbf{k}_i, \omega_i$  denote the polarization, time center, wavevector, and carrier frequency of the  $i$ -th pulse.  $E(t')$  is the slowly varying pulse envelope, which we choose to be Gaussian with fixed width  $\sigma$  for all pulses,  $E(t') = e^{-t'^2/2\sigma^2}$ . The polarization induced by the pulses on the molecule located at position  $\mathbf{r}$  is given by  $\mathbf{P}(\mathbf{r}, t') = \text{Tr}(\hat{\boldsymbol{\mu}}\rho(\mathbf{r}, t'))$ . This quantity can be Fourier decomposed along different wavevectors as  $\mathbf{P}(\mathbf{r}, t') = \sum_s \mathbf{P}_s(t') e^{i\mathbf{k}_s \cdot \mathbf{r}}$ , where the  $\mathbf{k}_s$  are linear combinations of wavevectors of the incoming fields. Radiation is produced due to the polarization (proportional to  $i\mathbf{P}(\mathbf{r}, t')$ ). We can choose to study a single component  $\mathbf{P}_s$  by detecting only the radiation moving in the direction  $\mathbf{k}_s$ . This is achieved by interfering the radiation with a fourth pulse moving in the direction  $\mathbf{k}_s$ , called the local oscillator (LO). In particular, we shall be interested in the time-integrated signal in the photon-echo (PE) direction,  $\mathbf{k}_4 = \mathbf{k}_{PE} = -\mathbf{k}_1 + \mathbf{k}_2 + \mathbf{k}_3$ . This heterodyne-detected signal  $[S_{PE}]_{\mathbf{e}_1, \mathbf{e}_2, \mathbf{e}_3, \mathbf{e}_4}^{\omega_1, \omega_2, \omega_3, \omega_4}$  is proportional to,

$$\int_{-\infty}^{\infty} dt' e^{i\omega_4(t' - t_4)} E(t' - t_4) \mathbf{e}_4 \cdot i\mathbf{P}_{PE}(t'), \quad (7)$$

where the subscripts indicate the polarizations of the four light pulses and the superscripts indicate their carrier frequencies. Spatial integration over the volume of probed molecules selects out the component  $\mathbf{P}_{PE}(t')$  from the  $\mathbf{P}(\mathbf{r}, t')$ . The time integration yields a signal that is proportional to the components of  $\mathbf{P}_{PE}(t') \cdot \mathbf{e}_4$  oscillating at the frequencies of the LO, which is centered about  $\omega_4$ .

. In this excitonic model, the only optically allowed transitions are between states differing by one excitation, so the only nonzero matrix elements of  $\hat{\boldsymbol{\mu}}$  are  $\boldsymbol{\mu}_{ij} = \boldsymbol{\mu}_{ji}$  for  $ij = \alpha g, \beta g, f\alpha, f\beta$  (SI-II).

In the following section, we present the main results of our study. We show that a carefully chosen set of two-color rephasing PE experiments can be used to perform a *QPT of the first exciton manifold* (Fig. 2). The preparation of initial states is achieved using the first two pulses at  $t_1$  and  $t_2$ . Initial states spanning the single exciton manifold are produced by using the four possible combinations of two different carrier frequencies for the first two pulses. In the terminology of PE experiments, these pulses define the so-called *coherence time* interval

$\tau = t_2 - t_1$ . The time interval between the second and third pulses, called the *waiting time*  $T = t_3 - t_2$ , defines the quantum channel which we want to characterize by QPT. Finally, we carry out QST of the output density matrix at the instant  $t_3$ . This task is indirectly performed by using the third pulse to selectively generate new dipole-active coherences, which are detected upon heterodyning with the fourth pulse at  $t_4$ , that is, after the *echo time*  $t = t_4 - t_3$  has elapsed. Varying the third and fourth pulse frequencies yields sufficient linear equations for QST. This procedure naturally concludes the protocol of the desired QPT.

## Results

For purposes of the QPT protocol, we assume that the structural parameters  $\omega_{\alpha g}$ ,  $\omega_{\beta g}$ ,  $\boldsymbol{\mu}_{\alpha g}$ ,  $\boldsymbol{\mu}_{\beta g}$ ,  $\boldsymbol{\mu}_{f\alpha}$ , and  $\boldsymbol{\mu}_{f\beta}$  are all known. Information about the transition frequencies can be obtained from a linear absorption spectrum, whereas the dipoles can be extracted from x-ray crystallography. As shown in recent work of our group, with enough data from the PE experiments, it is also possible to extract these parameters self-consistently. We proceed to describe the steps of the PE experiment on a coupled dimer that yield a QPT.

### Initial state preparation

Before any electromagnetic perturbation, the excitonic system is in the ground state  $\rho(-\infty) = |g\rangle\langle g|$ . After the first two pulses in the  $\mathbf{k}_1$ ,  $\mathbf{k}_2$  directions act on the system, the detected polarization will be determined by an effective density matrix  $\tilde{\rho}_{\mathbf{e}_1, \mathbf{e}_2}^{\omega_1, \omega_2}(0)$  (at  $T = 0$ ) which is second order in  $\lambda$ . By applying second order perturbation theory and the rotating-wave approximation (RWA), we can define an effective *initial state* (Fig. 3a–d, SI-III):

$$\begin{aligned} \tilde{\rho}_{\mathbf{e}_1, \mathbf{e}_2}^{\omega_1, \omega_2}(0) = & - \sum_{pq \in \{\alpha, \beta\}} C_{\omega_1}^p C_{\omega_2}^q (\boldsymbol{\mu}_{pg} \cdot \mathbf{e}_1) (\boldsymbol{\mu}_{qg} \cdot \mathbf{e}_2) \\ & \times \mathcal{G}_{gp}(\tau) (|q\rangle\langle p| - \delta_{pq} |g\rangle\langle g|). \end{aligned} \quad (8)$$

This state evolves during the waiting time  $T$  to give

$$\tilde{\rho}_{\mathbf{e}_1, \mathbf{e}_2}^{\omega_1, \omega_2}(T) = \chi(T) \tilde{\rho}_{\mathbf{e}_1, \mathbf{e}_2}^{\omega_1, \omega_2}(0), \quad (9)$$

which holds for  $T \gtrsim 3\sigma$ , that is, after the action of the first two pulses has effectively ended. Eq. 9 is of the form of Eq. 1, and therefore appealing for our QPT purposes. The purely imaginary coefficients  $C_{\omega_i}^p$  for  $p \in \{\alpha, \beta\}$  are proportional to the frequency components at  $\omega_{pg}$  of the pulse which is centered at  $\omega_i$ :

$$C_{\omega_i}^p = -\frac{\lambda}{i}\sqrt{2\pi\sigma^2}e^{-\sigma^2(\omega_{pg}-\omega_i)^2/2}, \quad (10)$$

and

$$\mathcal{G}_{ij}(\tau) = \Theta(\tau)e^{(-i\omega_{ij}-\Gamma_{ij})\tau} \quad (11)$$

is the propagator of the optical coherence  $|i\rangle\langle j|$ , which, for simplicity, has been taken to be the product of a coherent oscillatory term beating at a frequency  $\omega_{ij}$  and an exponential decay with dephasing rate  $\Gamma_{ij}$ , assumed to be known.  $\Theta(\tau)$  is the Heaviside function, so the propagator is finite only for times  $\tau \geq 0$ . We have kept only the  $-\mathbf{k}_1$  and  $+\mathbf{k}_2$  components because those are the only contributions to the signal at  $\mathbf{k}_{PE}$ .

Eq. (8) has a simple interpretation, and can be easily read off from the Feynman diagrams depicted in Fig. 3a–d. Since we will be selecting only light in the  $\mathbf{k}_{PE}$  direction, we keep only the portion of the first pulse proportional to  $e^{i\omega_1(t-t_1)}$  and only the portion of the second pulse proportional to  $e^{-i\omega_2(t-t_2)}$  in Eq. 6. Then, since the state before any perturbation is  $|g\rangle\langle g|$ , the first pulse can only resonantly excite the bra in the RWA, generating an optical coherence  $|g\rangle\langle p|$  (where  $p \in \{\alpha, \beta\}$ ) with amplitude  $C_{\omega_1}^p$ . This coherence undergoes free evolution for time  $\tau$  under  $\mathcal{G}_{gp}(\tau)$  before the second pulse perturbs the system. In the RWA, this second pulse can act on the ket of  $|g\rangle\langle p|$  to yield  $|q\rangle\langle p|$  with amplitude  $C_{\omega_2}^q$  and on the bra to create a *hole*  $-|g\rangle\langle g|$  with amplitude  $C_{\omega_2}^p$ , producing Eq. 8. The amplitude of this prepared initial state is proportional to the alignment of the corresponding transition dipole moments with the polarization of the incoming fields. Once the initial state is prepared, it evolves via  $\chi(T)$ , which is the object we want to characterize. A possible problem is the contamination of the initial states by terms proportional to a hole  $-|g\rangle\langle g|$  every time there is a single-exciton manifold population  $|p\rangle\langle p|$ . This is not a difficulty either if we assume:

$$\chi_{abgg}(T) = \delta_{ag}\delta_{bg}, \quad (12)$$

that is, if the ground state population does not transform into any other state via free evolution. This is reasonable since we may ignore processes where phonons can induce upward optical transitions. We similarly neglect spontaneous excitation from the single to double exciton states.

One can see from Eq. 8 that a set of four linearly independent initial states can be generated by manipulating the frequency components of the pulses through  $C_{\omega_1}^p$  and  $C_{\omega_2}^q$ . It is sufficient to consider a pulse toolbox of two waveforms which create  $|\alpha\rangle$  and  $|\beta\rangle$  with different amplitudes. For instance, by centering one waveform at  $\omega_+$  in the vicinity of  $\omega_{\alpha g}$  and the other at  $\omega_-$  close

to  $\omega_{\beta g}$ , we can simultaneously have:

$$\begin{aligned} C_{\omega_+}^{\alpha} &= C_{\omega_-}^{\beta} = C_1, \\ C_{\omega_+}^{\beta} &= C_{\omega_-}^{\alpha} = C_2, \end{aligned} \tag{13}$$

for purely imaginary numbers  $C_1 \neq C_2$ . The conceptually simplest choice, which we shall denote the *maximum discrimination choice* (MDC), and which is best for QPT purposes, is two waveforms each resonant with only one transition, so  $C_1 \gg C_2$ , and we can neglect  $C_2$ . Four linearly independent initial states can be prepared by choosing the waveform of each of the first two pulses from this pulse toolbox.

### Evolution

The system evolves during the waiting time  $T$  after the initial state is prepared. Transfers between coherences and populations are systematically described by  $\chi(T)$ . The components of  $\tilde{\rho}_{\mathbf{e}_1, \mathbf{e}_2}^{\omega_1, \omega_2}$  evolve in time, described by  $\chi(T)$ , without assuming any particular model for the bath or system-bath interaction, other than Eq. 12. By definition, the amplitude of the  $ij$  component of  $\tilde{\rho}_{\mathbf{e}_1, \mathbf{e}_2}^{\omega_1, \omega_2}(T)$  is proportional to  $\chi_{ijqp}(T)$ , with the exception of the  $gg$  component, which is proportional to  $\chi_{ggpq}(T) + \delta_{pq}$  due to the contamination of the hole in the initial state. We note that de-excitation transfers from the single-exciton manifold to elements involving the ground state ( $gg, g\alpha, g\beta$ ) are expected to be small, since such processes are also unlikely to occur on femtosecond timescales due to either the phonon or the photon bath. We will show that in our protocol we can detect decay into  $gg$  but not into  $g\alpha$  or  $g\beta$ . We shall keep these  $\chi_{ggqp}(T)$  terms in our equations in order to monitor *amplitude leakage errors* from the single-exciton manifold, providing a consistency check for treating the single-exciton manifold as an effective TLS in the timescale of interest. In case the experiment becomes much more difficult due to the inclusion of these terms, such terms could judiciously be set to zero without further changes in the theory.

### Detection

The last two pulses provide an indirect QST of the state after the waiting time. The third perturbation along  $+\mathbf{k}_3$  and centered at time  $t_3$  will selectively probe certain coherences and populations of  $\tilde{\rho}_{\mathbf{e}_1, \mathbf{e}_2}^{\omega_1, \omega_2}(T)$ . As an illustration (see Fig. 3e,f), the component of the pulse matching the transition energy  $\omega_{\alpha g} = \omega_{f\beta}$  and proportional to  $C_{\omega_3}^{\alpha}$  will, in the RWA, promote the resonant transitions  $|g\rangle \rightarrow |\alpha\rangle$  and  $|\beta\rangle \rightarrow |f\rangle$  on the ket side, and the conjugate resonant transitions

$\langle \alpha | \rightarrow \langle g |$  and  $\langle f | \rightarrow \langle \beta |$  on the bra side, the latter of which are irrelevant as we are ignoring transfers to the biexciton state during the waiting time. These transitions will generate two sets of optically active coherences in the echo interval:  $\alpha g$ ,  $f\beta$  which oscillate at frequency  $\omega_{\alpha g}$ , and  $\beta g$ ,  $f\alpha$  which oscillate at  $\omega_{\beta g}$ . These sets generate a polarization which interferes with the LO yielding signals proportional to  $C_{\omega_4}^\alpha$  and  $C_{\omega_4}^\beta$ , respectively. The propagator for the echo time is taken to be as in Eq. 11. A similar analysis can be repeated for the  $C_{\omega_3}^\beta$  term. Analogously to the preparation stage, the same toolbox of two different waveforms for the third and the fourth pulses allows discrimination of all final states of  $\tilde{\rho}_{e_1, e_2}^{\omega_1, \omega_2}(T)$ . Fig. 3 depicts double-sided Feynman diagrams for all possible combinations of preparations and detections with four pulses each chosen from two waveforms, yielding sixteen experiments. By keeping track of these processes, the signal  $[S_{PE}]_{e_1, e_2, e_3, e_4}^{\omega_1, \omega_2, \omega_3, \omega_4}$  may be compactly written as (SI-IV):

$$[S_{PE}]_{e_1, e_2, e_3, e_4}^{\omega_1, \omega_2, \omega_3, \omega_4}(\tau, T, t) \propto \sum_{p, q, r, s} C_{\omega_1}^p C_{\omega_2}^q C_{\omega_3}^r C_{\omega_4}^s P_{e_1, e_2, e_3, e_4}^{p, q, r, s}(\tau, T, t), \quad (14)$$

where the proportionality constant is purely real, and the expression holds for  $T, t > 3\sigma$ . The terms  $P_{e_1, e_2, e_3, e_4}^{p, q, r, s}(\tau, T, t)$  are loosely polarizations (in fact, they are proportional to  $i$  times polarizations) and are given by

$$\begin{aligned} & P_{e_1, e_2, e_3, e_4}^{p, q, \alpha, \alpha}(\tau, T, t) \\ &= -(\boldsymbol{\mu}_{pg} \cdot \mathbf{e}_1)(\boldsymbol{\mu}_{qg} \cdot \mathbf{e}_2)\mathcal{G}_{gp}(\tau) \\ & \quad \times \{[(\boldsymbol{\mu}_{\alpha g} \cdot \mathbf{e}_3)(\boldsymbol{\mu}_{\alpha g} \cdot \mathbf{e}_4)\mathcal{G}_{\alpha g}(t) \\ & \quad \times (\chi_{ggqp}(T) - \delta_{pq} - \chi_{\alpha\alpha qp}(T)) \\ & \quad + (\boldsymbol{\mu}_{f\beta} \cdot \mathbf{e}_3)(\boldsymbol{\mu}_{f\beta} \cdot \mathbf{e}_4)\mathcal{G}_{f\beta}(t)\chi_{\beta\beta qp}(T)]\}, \end{aligned} \quad (15)$$

and

$$\begin{aligned} & P_{e_1, e_2, e_3, e_4}^{p, q, \alpha, \beta}(\tau, T, t) \\ &= -(\boldsymbol{\mu}_{pg} \cdot \mathbf{e}_1)(\boldsymbol{\mu}_{qg} \cdot \mathbf{e}_2)\mathcal{G}_{gp}(\tau) \\ & \quad \times \{[(\boldsymbol{\mu}_{f\beta} \cdot \mathbf{e}_3)(\boldsymbol{\mu}_{f\alpha} \cdot \mathbf{e}_4)\mathcal{G}_{f\alpha}(t) \\ & \quad - (\boldsymbol{\mu}_{\alpha g} \cdot \mathbf{e}_3)(\boldsymbol{\mu}_{\beta g} \cdot \mathbf{e}_4)\mathcal{G}_{\beta g}(t)]\chi_{\beta\alpha qp}(T)]\}. \end{aligned} \quad (16)$$

The remaining terms  $P_{e_1, e_2, e_3, e_4}^{p, q, \beta, \beta}(\tau, T, t)$ ,  $P_{e_1, e_2, e_3, e_4}^{p, q, \beta, \alpha}(\tau, T, t)$  follow upon the interchange  $\alpha \leftrightarrow \beta$ . Eqs. 14-16 are the main result of this article. Each  $P_{e_1, e_2, e_3, e_4}^{p, q, r, s}$  represents the observed signal if the first (second, third, fourth) laser pulse is resonant only with the  $p$  ( $q, r, s$ ) transition. The total measured signal  $[S_{PE}]_{e_1, e_2, e_3, e_4}^{\omega_1, \omega_2, \omega_3, \omega_4}(\tau, T, t)$  is a weighted sum of these  $P_{e_1, e_2, e_3, e_4}^{p, q, r, s}$ . Equations



15,16 show that each  $P_{\mathbf{e}_1, \mathbf{e}_2, \mathbf{e}_3, \mathbf{e}_4}^{p,q,r,s}$  is a linear combination of elements of  $\chi(T)$ , corresponding to the prepared initial states and detected final states. After collecting the sixteen signals  $[S_{PE}]_{\mathbf{e}_1, \mathbf{e}_2, \mathbf{e}_3, \mathbf{e}_4}^{\omega_1, \omega_2, \omega_3, \omega_4}$  with each pulse carrier frequency  $\omega_i$  chosen from  $\{\omega_+, \omega_-\}$  as in Eq. (13), with fixed polarizations  $\mathbf{e}_i$ , Eq. (14) can be inverted to yield the elements of  $\chi(T)$  associated with the single-exciton manifold of the dimer, hence accomplishing the desired QSTs and QPT at once. Notice that in principle, for a given value of waiting time  $T$ , the one-dimensional (1D) measurements associated with a single set of  $\tau, t$  values is enough for purposes of QPT of the single exciton manifold. In the most typical measurements, the sample has isotropically distributed chromophores, so Eq. 14 must be modified to include isotropic averaging  $\langle \cdot \rangle_{\text{iso}}$  (SI-VI). Since the present QPT protocol does not rely on different polarization settings, we will assume for simplicity that each of the sixteen experiments is carried out with  $(\mathbf{e}_1, \mathbf{e}_2, \mathbf{e}_3, \mathbf{e}_4) = (z, z, z, z)$ . Further technical details of the QPT protocol can be found in the next section as well as in SI-V–XI.

### Important observations

(a) DIFFERENCE BETWEEN A STANDARD PE EXPERIMENT AND QPT. In the current practice of NLOS, model Hamiltonians with free parameters for the excitonic system, the bath, and the interaction between them are postulated, and the experimental spectra are fit to the model via calculation of response functions, from which structural and dynamical information is extracted. In our language, such experiments involve fitting models to complicated combinations of quantum processes associated with  $\chi(T)$ . QPT requires only a model for the excitonic system, but not for the bath or the system-bath coupling, making it suitable for probing systems where the bath dynamics are unknown. By definition, QPT extracts the elements of  $\chi(T)$ , allowing a straightforward analysis of processes directly associated with the density matrix, such as dephasing and relaxation.

(b) QPT CAN ALSO BE PERFORMED WITH CONTROL OF TIME DELAYS  $\tau, t$  INSTEAD OF FREQUENCY CONTROL. Although 1D measurements suffice for QPT, suppose the signal is collected for many values of  $\tau$  and  $t$ . Upon appropriately defined Fourier transformations of the signal along these variables, a two-dimensional electronic spectrum (2D-ES) can be constructed where the coherence propagators of Eq. (11) manifest as four resonances about  $\omega_{\alpha g}$  and  $\omega_{\beta g}$  along both axes. An important observation follows: the frequencies of the coherent evolutions in the coherence and echo times are the same as the frequencies of the first transition and the LO detection. By varying  $t$  and  $\tau$ , a 2D-ES provides the frequency-controlled information of the first and fourth pulses. Hence, it is possible to make the first and fourth pulses sufficiently

broadband that they excite both  $\alpha$  and  $\beta$  with similar magnitude. Then, the sixteen 1D experiments can be replaced with four 2D-ES where the second and third pulses are frequency controlled. A caveat in this identification is the assumption that the optical coherences evolve in a form like Eq. 11, without errors of coherence transfers (SI-VII,IX).

(c) EXTENSION TO OVERLAPPING PULSES. The discussion above assumed negligible pulse overlaps. Remarkably, Eqs. (14), (15) and (16) still hold if  $\tau, t \geq 0$  and  $T > 3\sigma$ , with the exception that  $C_{\omega_3}^r C_{\omega_4}^s$  in Eq. 14 must be replaced by

$$C_{\omega_3}^r C_{\omega_4}^s \frac{1}{2} \left[ 1 + \text{Erf} \left( \frac{t}{2\sigma} + \frac{i(\omega_3 - \omega_{rg} + \omega_4 - \omega_{sg})\sigma}{2} \right) \right] \quad (17)$$

to account for the fact that the third pulse must act in the sample *before* the LO can detect the polarization (SI-IV-B). In the case of well-separated pulses,  $t \gg \sigma$ , Eq. 17 reduces to  $C_{\omega_3}^r C_{\omega_4}^s$ .

The measurements of the real and imaginary part of the PE signal in the  $\tau, t = 0$  limit are recognized with the names of transient dichroism (TD) and transient birefringence (TB), respectively, and are very interesting for QPT. For resonant TD/TB ( $\omega_3 + \omega_4 = \omega_{rs} + \omega_{sg}$ ), Eq. (17) reduces to  $\frac{1}{2} C_{\omega_3}^r C_{\omega_4}^s$ , which shows that the LO monitors only half of the original polarization since it interferes with the polarization as it is generated. Consider such a resonant TD/TB experiment where, even though the pulses can achieve frequency selectivity, they are short in the sense that  $\sigma \ll \frac{1}{\lambda}$ , where  $\lambda$  is a characteristic reorganization energy scale of the bath. In this situation, the bath state will not evolve during the pulse duration, allowing unambiguous preparation of initial excitonic states tensored with the *same* equilibrium bath configuration (SI-VIII), yielding a consistent QPT. Also, for  $\tau, t = 0$ , the free evolution of the optical coherences does not contribute to the signal, and the short timescale  $\sigma$  does not allow for errors of population or coherence transfers to occur in the preparation or detection stages. Hence, a highlight of the TD/TB signal is that it is determined exclusively by the dynamics of the single-exciton manifold. Scenarios where the TD/TB configuration is preferred compared to the PE are excitonic systems coupled to highly non-Markovian baths.

(d) NUMERICAL STABILITY OF QPT. An investigation of the stability properties of the matrices associated with the reconstruction of  $\chi(T)$  from the sixteen enumerated experiments shows that our protocol is very robust upon the variation of the structural parameters of the system, namely, the ratio between the two dipole norms  $d_B/d_A$ , the angle between the site dipoles  $\phi$ , and the mixing angle  $\theta$ . General exceptions occur at the vicinity of  $\theta = 0, \frac{\pi}{2}$  where the coupling  $J$  vanishes, as well as for  $\theta = \frac{\pi}{4}, \frac{3\pi}{4}$  and  $d_B/d_A = 1$ , that is, the homodimer case (SI-XI-A and B).

(e) SCALABILITY. The ideas presented in the article can be easily extended to general multi-chromophoric systems, where the pulse toolbox consists of  $d$  different waveforms for an aggregate

consisting of  $d$  chromophores (the relevant Hilbert space is the single exciton manifold, which is of size  $d$ ). Let us make a crude comparison of the number of resources required to accomplish a multichromophoric QPT with respect to a standard 2D-ES. Contrasting the number of experiments in one setting with respect to another does not necessarily provide a fair estimate of the real effort, as an experimentalist might have built a machine that efficiently carries one type of measurement, but not the other. However, at least this estimate gives an idea of the resources involved in each situation. On the one hand, without keeping track of leakage errors, the number of required 1D experiments for a QPT is just equal to the number of parameters to extract,  $d^4 - d^2$ . On the other hand, the number of grid points in a single 2D-ES, which we take as equivalent to the effective number of performed experiments, is on the order of 7000. Therefore, it is only for  $d > 10$  that a QPT becomes more costly than a single 2D-ES in terms of the number of experiments. Clearly, the scalability of QPT as  $O(d^4)$  is not favorable asymptotically, although ideas associated with single shot setups should not be discarded. However, this limit might not even be relevant for the current state of the art experiments. So far, the largest multichromophoric system for which the spectral lineshapes can be resolved in a 2D-ES consists of the lowest lying states of the Light Harvesting Complex-II, corresponding to  $d = 14$ , giving  $14^4 - 14^2 = 38220$  1D experiments, which amounts to a similar effort to collecting approximately six 2D-ES. In any case, it would still be interesting to start developing ways to perform compressed QPT protocols for energy transfer systems large enough that the protocol suggested here would be impractical (see for recent ideas on scalable QPTs).

### Numerical example

To test the extraction of  $\chi$  from experimental spectra, we consider a dimer with Hamiltonian parameters that are on the order of previously reported experiments consisting of light harvesting systems ( $\omega_A = 12881 \text{ cm}^{-1}$ ,  $\omega_B = 12719 \text{ cm}^{-1}$ ,  $J = 120 \text{ cm}^{-1}$ , yielding  $\theta = 0.49$ ). We assume a toolbox of two carrier frequencies  $\omega_+ = 13480 \text{ cm}^{-1}$  and  $\omega_- = 12130 \text{ cm}^{-1}$ , respectively, so that  $\omega_i \in \{\omega_+, \omega_-\}$  for all  $i$ , and the width of the pulses to be  $FWHM = 40 \text{ fs}$ , which corresponds to  $\sigma = 17 \text{ fs}$ . The parameters satisfy the MDC condition with  $C_1/C_2 = 20$ . The pulses are long enough to guarantee the selectivity of the produced exciton, but short enough to allow for the evolution of the bath induced excitonic dynamics to be monitored. We choose  $d_B/d_A = 2$  and  $\phi = 0.3$ . We present simulations on the QPT for this system, where each chromophore is linearly coupled to an independent Markovian bath of harmonic oscillators. The dissipative effects are modeled through a secular Redfield model at temperature  $\underline{T} = 273 \text{ K}$  (SI-X).

Since we are working in the MDC regime, the signals in Eq. 14 are simply proportional to  $\langle P_{\mathbf{e}_1, \mathbf{e}_2, \mathbf{e}_3, \mathbf{e}_4}^{p,q,r,s}(\tau, T, t) \rangle_{iso}$ . Fig. 4 plots the sixteen real and imaginary parts of the  $\langle P_{z,z,z,z}^{p,q,r,s}(0, T, 0) \rangle_{iso}$  values, which can be regarded as signals from the TD/TB setting, or as PE signals with the coherence and echo time propagators factored out. They have been calculated via an isotropic average of Eq. (15) and (16) (SI-VI,XI-B). In our simulations, we consider an inhomogeneously broadened ensemble of 10,000 dimers with diagonal disorder. The site energies are drawn from Gaussian distributions centered about  $\omega_A$  and  $\omega_B$ , respectively, both with standard deviation of  $\sigma_{inh} = 40 \text{ cm}^{-1}$ . For every waiting time  $T$ , the signal is calculated with this fixed ensemble. After a normalization step, the signals are of  $O(1)$  or smaller. Additional noise simulating experimental errors due to laser fluctuations is included. This consists of independent realizations at every waiting time  $T$  of Gaussian noise on the measured signals with zero mean and  $\sigma_{laser} = 0.05$  standard deviation.

Fig. 4 plots the ideal and inhomogeneously broadened, noisy signals as continuous and discrete points, respectively. The ideal signals are calculated from a single dimer with no disorder and without laser fluctuations. All plots start at  $T = 3\sigma = 51 \text{ fs}$ , since for earlier times, the initial states are not yet effectively prepared. Errors in experimental signals  $\langle P_{z,z,z,z}^{p,q,r,s}(0, T, 0) \rangle_{iso}$  translate into errors of reconstructed  $\chi(T)$ . An estimate of the amplification of relative errors is set by the condition numbers of the matrices to be inverted, which is lower than  $\kappa = 2.9$  for our set of parameters  $d_B/d_A$ ,  $\theta$ ,  $\phi$  (SI-XI-B). Reconstruction of  $\chi$  must respect the known symmetries, Eqs. 2-4. Eqs. 2-3 are built into the corresponding matrix equations, but Eq. (4) must be included by using a semidefinite programming routine. The latter is implemented using the open-source package CVX, and the result is Fig. 5, which shows the discrete points representing the reconstructed elements of  $\chi(T)$  from noisy data on top of the ideal results plotted as continuous functions of  $T$ . Notice the remarkable agreement between the ideal and the reconstructed results, despite the significant inhomogeneous broadening and noise. The relative error of the inverted  $\chi(T)$  averages to 0.12.

Fig. 5 illustrates the final objective of a coupled dimer QPT, namely, the process matrix  $\chi(T)$ . Each panel shows processes of the density matrix as a function of  $T$ , conditional on the initial state being  $\alpha\alpha$  (a),  $\beta\beta$  (b), and  $\alpha\beta$  (c and d), with the ideal  $T$ -dependence. The detailed balance condition in the Redfield model implies that  $\chi_{\beta\beta\alpha\alpha} = \chi_{\alpha\alpha\beta\beta} e^{\omega_{\alpha\beta}/k_B T}$ , which can be seen in panels (a) and (b). Also, note that due to the secular approximation, coherence-to-population and the reverse processes are zero. Note that all the decoherence processes in our model occur within a timescale of hundreds of femtoseconds, with the  $\alpha\beta$  coherence evolving through about three periods before practically vanishing (c and d). Clearly, a more complex interplay of the excitonic system with the phonon bath is possible, but this example illustrates

the essence of the type of information which can be obtained through QPT.

## Conclusions

In this article, we have introduced QPT as a powerful tool to systematically characterize the dynamics of excitonic systems in condensed phases. We identified the coherence, waiting, and echo intervals of the PE experiment with the state preparation, free evolution, and detection stages of a QPT. In order to achieve selective state preparation and detection, we suggested frequency control through pulses of two different colors, although scenarios with time delays and pulse polarizations as control knobs were also discussed here and elsewhere . By choosing between these colors for each of the four pulses, sixteen experiments can be carried out, which yield all the elements of  $\chi(T)$  related to the single-exciton manifold. An analysis of the reconstruction of  $\chi(T)$  in the presence of inhomogeneous broadening and experimental noise was provided, and the simulation on a model system shows that QPT of an excitonic system in condensed phase is a very plausible goal.

Equipped with  $\chi(T)$ , which completely characterizes the excitonic dynamics, a plethora of questions can be rigorously answered about it. Some examples are: Can the bath be described as Markovian? If so, does the secular approximation hold, or can a population spontaneously be transferred to a coherence? If not, what is its degree of non-Markovianity? Does a given master equation accurately describe the dynamics of the system? What is the timescale of each decoherence process? Are the baths coupled to each chromophore correlated? How much entanglement is induced in the system upon photoexcitation? Once these questions are answered, interesting questions of control and manipulation of excitons can be asked.

In summary, a QIP approach to nonlinear spectroscopy via QPT offers novel insights on the ways to design experiments in order to extract information about the quantum state of the energy transfer system. We believe this work bridges a gap between theoretical and experimental studies on excitation energy transfer from the QIP and physical chemistry communities, respectively.

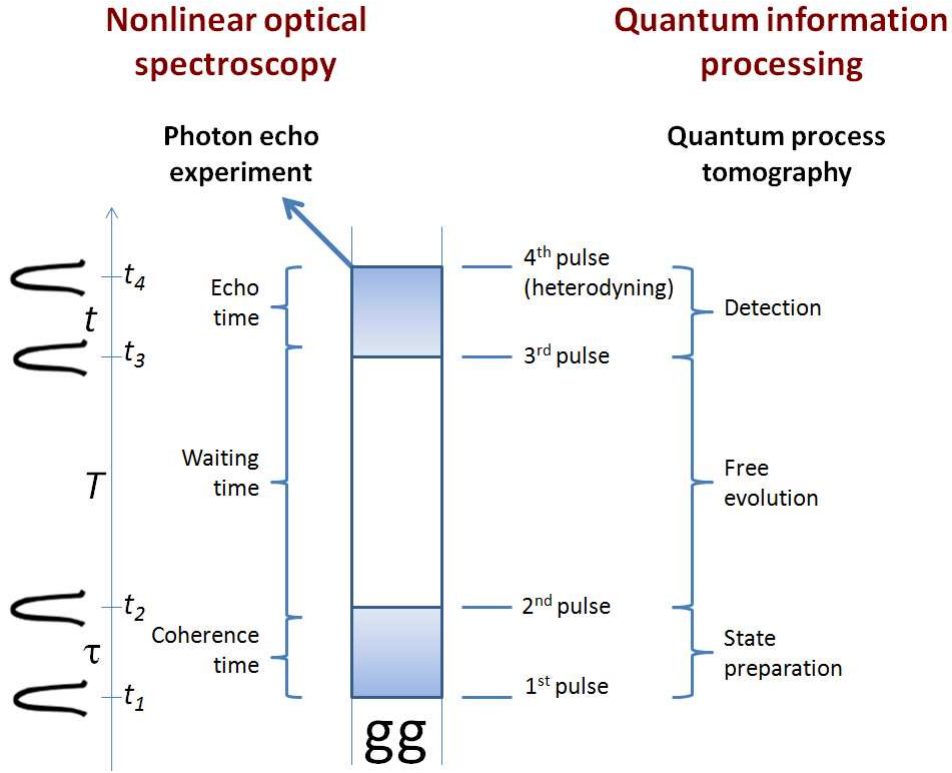

Figure 1: A set of photon echo experiments can be regarded as a QPT. Pulses are centered about  $t_1, t_2, t_3, t_4$ . Time flows upwards in the diagram. The four pulses define the *coherence* ( $\tau$ ), *waiting* ( $T$ ) times, and *echo* ( $t$ ) times. This experiment, in the language of quantum information processing, can be regarded as consisting of three stages: initial state preparation, free evolution, and detection of the output state of the waiting time.

## Acknowledgements

We acknowledge stimulating discussions with Hohjai Lee, Dylan Arias, Patrick Wen, and Keith Nelson. This work was supported by the Center of Excitonics, US Department of Energy, Award Number DESC0001088. Support from the Harvard University Center for the Environment is also acknowledged.

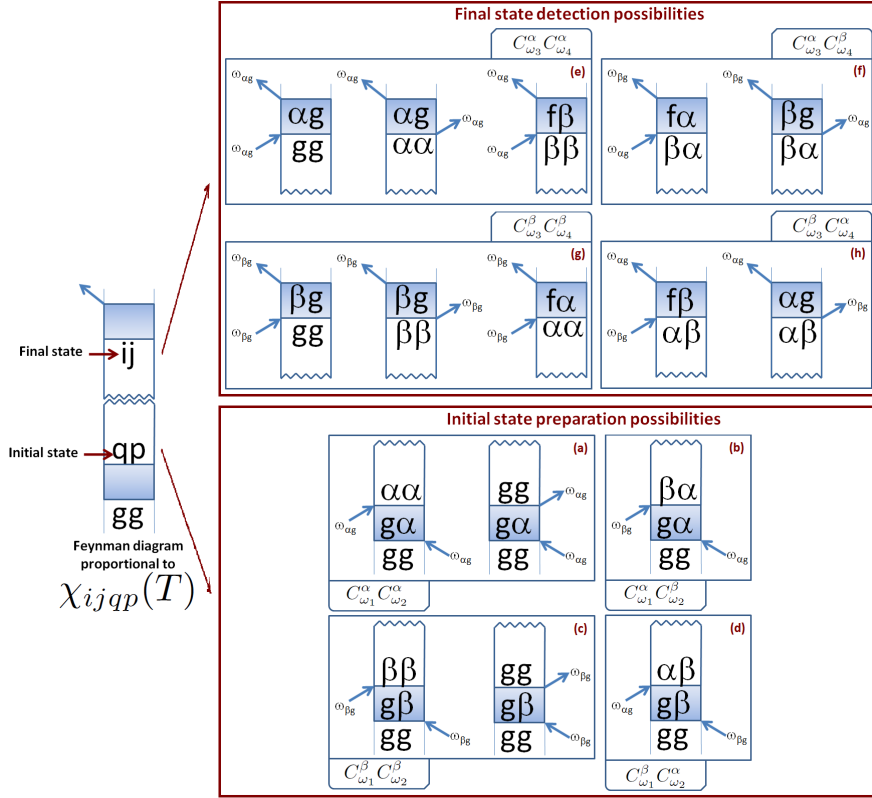

Figure 2: *Possible state preparations and detections.* We list all the possible preparations and detections of elements of the density matrix of the waiting time  $T$  via a rephasing PE experiment. The double sided Feynman diagrams above list all the possible processes detected in a rephasing PE experiment. Each diagram is related to an element  $\chi_{ijqp}(T)$  due to the prepared state  $|q\rangle\langle p| - \delta_{pq}|g\rangle\langle g|$  at the beginning of the waiting time and the detected state  $ij$  at the end of it. By combining the preparations in (a), (b), (c), and (d), with the detections in (e), (f), (g), and (h), sixteen different types of processes can be enumerated, which can be classified according to the pulse frequencies of the associated perturbations.

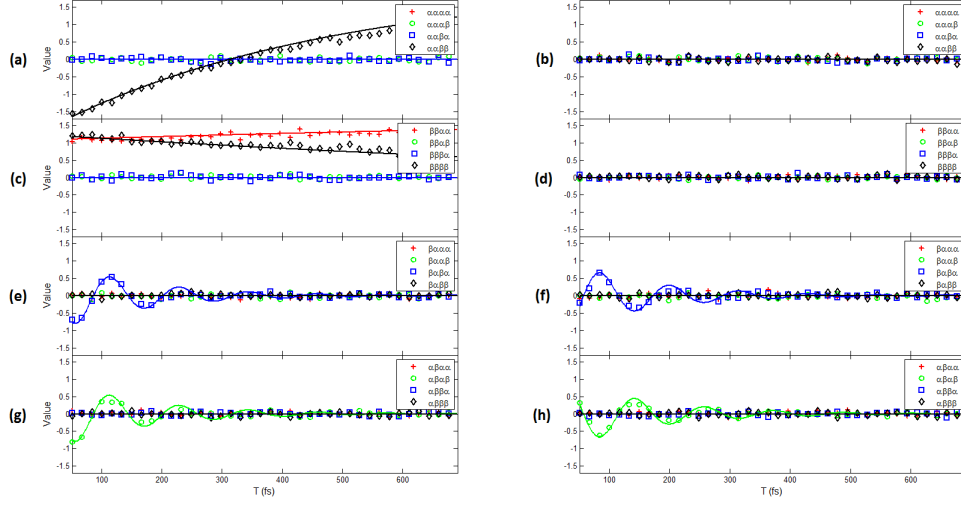

Figure 3: *Real (a,c,e,g) and imaginary (b,d,f,h) parts of polarization signals from sixteen two-color experiments for fixed  $\tau = t = 0$ . The legends  $pqrs$  correspond to the real (left) and imaginary (right) parts of the isotropically averaged signals  $\langle P_{z,z,z,z}^{p,q,r,s}(0,T,0) \rangle_{iso}$ . The panels are organized by QPT initial state ((a) and (b) for  $|\alpha\rangle\langle\alpha|$ , (c) and (d) for  $|\beta\rangle\langle\beta|$ , (e) and (f) for  $|\alpha\rangle\langle\beta|$ , and (g) and (h) for  $|\beta\rangle\langle\alpha|$ ). The ideal signals are depicted as continuous functions whereas the simulations with disorder and experimental noise are represented as discrete points of the same color.*

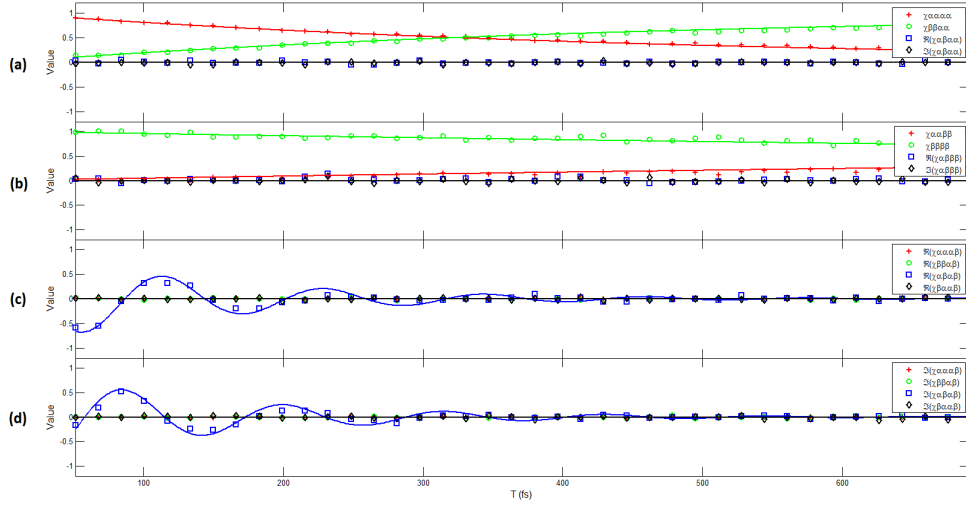

Figure 4: *Elements of  $\chi(T)$  for the numerical example. The true values are shown as a continuous function, whereas the discrete points represent the extraction from noisy data. The panels are organized according to the initial state, (a) for  $|\alpha\rangle\langle\alpha|$ , (b) for  $|\beta\rangle\langle\beta|$ , and (c) and (d) for  $|\alpha\rangle\langle\beta|$ .*



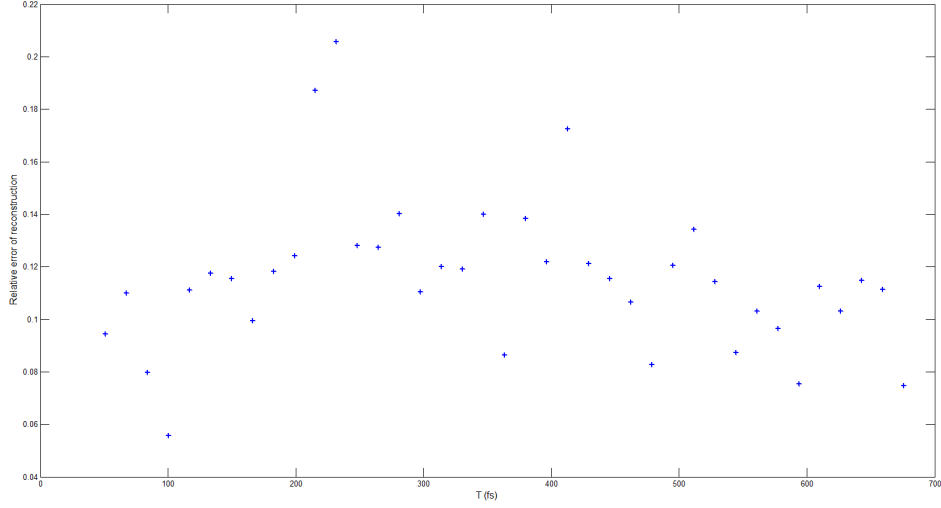

Figure 5: *Relative errors of  $\chi(T)$  extraction as a function of waiting time  $T$ . The errors of the reconstruction average to a value of 0.12.*

Table 1. A set of experiments which yields  $\chi(T)$

| From the data                                                                                                                                                                                                                                                                                                                                                                                                                                                                                                                                                                                                                                                                               | we can reconstruct the elements                             | which explicitly listed are                                                                                                                                                                                                                                                                                                                                                                                                                                                                                                                                                                                                                                                                                                                                     |
|---------------------------------------------------------------------------------------------------------------------------------------------------------------------------------------------------------------------------------------------------------------------------------------------------------------------------------------------------------------------------------------------------------------------------------------------------------------------------------------------------------------------------------------------------------------------------------------------------------------------------------------------------------------------------------------------|-------------------------------------------------------------|-----------------------------------------------------------------------------------------------------------------------------------------------------------------------------------------------------------------------------------------------------------------------------------------------------------------------------------------------------------------------------------------------------------------------------------------------------------------------------------------------------------------------------------------------------------------------------------------------------------------------------------------------------------------------------------------------------------------------------------------------------------------|
| $\left\{ \begin{array}{l} \langle P^{\alpha,\alpha,\alpha,\alpha}_{z,z,z,z}(\tau, T, t) \rangle_{iso}, \\ \langle P^{\alpha,\alpha,\alpha,\beta}_{z,z,z,z}(\tau, T, t) \rangle_{iso}, \\ \langle P^{\alpha,\alpha,\beta,\beta}_{z,z,z,z}(\tau, T, t) \rangle_{iso}, \\ \langle P^{\alpha,\alpha,\beta,\alpha}_{z,z,z,z}(\tau, T, t) \rangle_{iso} \end{array} \right\}$                                                                                                                                                                                                                                                                                                                     | $\{\chi_{ij\alpha\alpha}(T)\}$                              | $\left\{ \begin{array}{l} \chi_{\alpha\alpha\alpha\alpha}(T), \\ \chi_{\beta\beta\alpha\alpha}(T), \\ \Re\{\chi_{\alpha\beta\alpha\alpha}(T)\} = \Re\{\chi_{\beta\alpha\alpha\alpha}(T)\}, \\ \Im\{\chi_{\alpha\beta\alpha\alpha}(T)\} = -\Im\{\chi_{\beta\alpha\alpha\alpha}(T)\} \end{array} \right\}$                                                                                                                                                                                                                                                                                                                                                                                                                                                        |
| $\left\{ \begin{array}{l} \langle P^{\beta,\beta,\alpha,\alpha}_{z,z,z,z}(\tau, T, t) \rangle_{iso}, \\ \langle P^{\beta,\beta,\alpha,\beta}_{z,z,z,z}(\tau, T, t) \rangle_{iso}, \\ \langle P^{\beta,\beta,\beta,\beta}_{z,z,z,z}(\tau, T, t) \rangle_{iso}, \\ \langle P^{\beta,\beta,\alpha,\beta}_{z,z,z,z}(\tau, T, t) \rangle_{iso} \end{array} \right\}$                                                                                                                                                                                                                                                                                                                             | $\{\chi_{ij\beta\beta}(T)\}$                                | $\left\{ \begin{array}{l} \chi_{\alpha\alpha\beta\beta}(T), \\ \chi_{\beta\beta\beta\beta}(T), \\ \Re\{\chi_{\alpha\beta\beta\beta}(T)\} = \Re\{\chi_{\beta\alpha\beta\beta}(T)\}, \\ \Im\{\chi_{\alpha\beta\beta\beta}(T)\} = -\Im\{\chi_{\beta\alpha\beta\beta}(T)\} \end{array} \right\}$                                                                                                                                                                                                                                                                                                                                                                                                                                                                    |
| $\left\{ \begin{array}{l} \langle P^{\beta,\alpha,\alpha,\alpha}_{z,z,z,z}(\tau, T, t) \rangle_{iso}, \\ \langle P^{\beta,\alpha,\alpha,\beta}_{z,z,z,z}(\tau, T, t) \rangle_{iso}, \\ \langle P^{\beta,\alpha,\beta,\beta}_{z,x,x,z}(\tau, T, t) \rangle_{iso}, \\ \langle P^{\beta,\alpha,\beta,\alpha}_{z,x,x,z}(\tau, T, t) \rangle_{iso}, \\ \langle P^{\alpha,\beta,\alpha,\alpha}_{z,z,z,z}(\tau, T, t) \rangle_{iso}, \\ \langle P^{\alpha,\beta,\alpha,\beta}_{z,z,z,z}(\tau, T, t) \rangle_{iso}, \\ \langle P^{\alpha,\beta,\beta,\beta}_{z,z,z,z}(\tau, T, t) \rangle_{iso}, \\ \langle P^{\alpha,\beta,\beta,\alpha}_{z,z,z,z}(\tau, T, t) \rangle_{iso} \end{array} \right\}$ | $\{\chi_{ij\alpha\beta}(T) = (\chi_{ji\beta\alpha}(T))^*\}$ | $\left\{ \begin{array}{l} \Re\{\chi_{\alpha\alpha\alpha\beta}(T)\} = \Re\{\chi_{\alpha\alpha\beta\alpha}(T)\}, \\ \Im\{\chi_{\alpha\alpha\alpha\beta}(T)\} = -\Im\{\chi_{\alpha\alpha\beta\alpha}(T)\}, \\ \Re\{\chi_{\beta\beta\alpha\beta}(T)\} = \Re\{\chi_{\beta\beta\beta\alpha}(T)\}, \\ \Im\{\chi_{\beta\beta\alpha\beta}(T)\} = -\Im\{\chi_{\beta\beta\beta\alpha}(T)\}, \\ \Re\{\chi_{\alpha\beta\alpha\beta}(T)\} = \Re\{\chi_{\beta\alpha\beta\alpha}(T)\}, \\ \Im\{\chi_{\alpha\beta\alpha\beta}(T)\} = -\Im\{\chi_{\beta\alpha\beta\alpha}(T)\}, \\ \Re\{\chi_{\beta\alpha\alpha\beta}(T)\} = \Re\{\chi_{\alpha\beta\beta\alpha}(T)\}, \\ \Im\{\chi_{\beta\alpha\alpha\beta}(T)\} = -\Im\{\chi_{\alpha\beta\beta\alpha}(T)\} \end{array} \right\}$ |

---

TABLE 2. Values (in ps<sup>-1</sup>) of non-zero rates of the (secular) Redfield tensor at  $\underline{T} = 273$  K

---

|                                                                                                       |       |
|-------------------------------------------------------------------------------------------------------|-------|
| $R_{\beta\beta\alpha\alpha}$                                                                          | 2.15  |
| $R_{\alpha\alpha\beta\beta} = e^{-\omega_{\alpha\beta}/k_B \underline{T}} R_{\beta\beta\alpha\alpha}$ | 0.467 |
| $R_{\alpha\beta\alpha\beta} = R_{\beta\alpha\beta\alpha}$                                             | 6.91  |
| $R_{\alpha g \alpha g} = R_{g \alpha g \alpha} = R_{f \alpha f \alpha} = R_{\alpha f \alpha f}$       | 6.95  |
| $R_{\beta g \beta g} = R_{g \beta g \beta} = R_{f \beta f \beta} = R_{\beta f \beta f}$               | 6.11  |
| $R_{f g f g} = R_{g f g f}$                                                                           | 17.9  |

---



---

TABLE 3. Analytical expressions for the nonzero elements of  $\chi(T)$  involving single-exciton states

---

|                                                                           |                                                                |
|---------------------------------------------------------------------------|----------------------------------------------------------------|
| $\chi_{\alpha\alpha\alpha\alpha}(T)$                                      | $e^{-R_{\beta\beta\alpha\alpha}T}$                             |
| $\chi_{\beta\beta\alpha\alpha}(T)$                                        | $1 - e^{-R_{\beta\beta\alpha\alpha}T}$                         |
| $\chi_{\beta\beta\beta\beta}(T)$                                          | $e^{-R_{\alpha\alpha\beta\beta}T}$                             |
| $\chi_{\alpha\alpha\beta\beta}(T)$                                        | $1 - e^{-R_{\alpha\alpha\beta\beta}T}$                         |
| $\chi_{\alpha\beta\alpha\beta}(T) = (\chi_{\beta\alpha\beta\alpha}(T))^*$ | $e^{-i\omega_{\alpha\beta}T} e^{-R_{\alpha\beta\alpha\beta}T}$ |

---

# Quantum State and Process Tomography of Energy Transfer Systems via Ultrafast Spectroscopy

## *Supporting Information*

Joel Yuen-Zhou, Jacob J. Krich, Masoud Mohseni and Alán Aspuru-Guzik

## Contents

- I.** PROPERTIES OF  $\chi(T)$ . DERIVATION OF EQUATIONS 1-4 IN THE ARTICLE
- II.** TRANSITION DIPOLES OF THE COUPLED DIMER MODEL
- III.** STATE PREPARATION. DERIVATION OF EQUATION 9 IN THE ARTICLE
  - A.** WELL-SEPARATED PULSES 1 AND 2
  - B.** OVERLAPPING PULSES 1 AND 2
- IV.** STATE DETECTION. DERIVATION OF EQUATIONS 14-16 IN THE ARTICLE
  - A.** WELL-SEPARATED PULSES 3 AND 4
  - B.** OVERLAPPING PULSES 3 AND 4
- V.** OVERALL MULTIPLICATIVE CONSTANT
- VI.** ISOTROPIC AVERAGES
- VII.** ERRORS IN STATE PREPARATION AND DETECTION
- VIII.** DISCUSSION OF THE FACTORIZABLE CONDITION AT  $T = 0$
- IX.** TRADING FREQUENCY CONTROL FOR TIME DELAY
- X.** SECULAR REDFIELD MODEL FOR MARKOVIAN DISSIPATION
- XI.** RECONSTRUCTION OF  $\chi(T)$ 
  - A.** RECONSTRUCTION OF THE VALUES  $\langle P_{z,z,z,z}^{p,q,r,s}(\tau, T, t) \rangle_{iso}$  FROM THE SIGNALS  $\langle [S_{PE}]_{z,z,z,z}^{\omega_1, \omega_2, \omega_3, \omega_4}(\tau, T, t) \rangle_{iso}$

**B.** RECONSTRUCTION OF  $\chi(T)$  FROM  $\langle P_{z,z,z,z}^{p,q,r,s}(\tau, T, t) \rangle_{iso}$

**C.** CHOOSING SIXTEEN MEASUREMENTS OUT OF THE THIRTY-TWO HETERODYNE DETECTIONS

**XII.** SCALABILITY

## I. PROPERTIES OF $\chi(T)$ . DERIVATION OF EQUATIONS 1-4 IN THE ARTICLE

PROOF OF EQ. 1 IN THE ARTICLE.— Consider a system  $S$  that interacts with a bath  $B$ . Denote the total density matrix of the composite object as  $\rho_{\text{total}}$ , and the reduced density matrices for the system and the bath as  $\rho$  and  $\rho_B$ , respectively. That is,  $\rho = \text{Tr}_B \rho_{\text{total}}$ , where the trace is over the degrees of freedom of the bath, and similarly for  $\rho_B$ . Assume that the initial state of  $\rho_{\text{total}}$  is a tensor product form,

$$\rho_{\text{total}}(0) = \rho(0) \otimes \rho_B(0), \quad (\text{S1})$$

where  $\rho_B(0)$  is always

$$\rho_B(0) = \sum_{\beta} p_{\beta} |e_{\beta}\rangle \langle e_{\beta}|, \quad (\text{S2})$$

for every initial state  $\rho(0)$  of the system, with  $p_{\beta} \geq 0$  and  $\sum_{\beta} p_{\beta} = 1$ . At time  $T$ , the total state is a unitary evolution of the initial total state,

$$\rho_{\text{total}}(T) = U(T) \rho(0) \otimes \rho_B(0) U^{\dagger}(T). \quad (\text{S3})$$

Here,  $U(T) = \mathcal{T}(e^{-i \int_0^T H_{\text{total}}(t') dt'})$  is the propagator for the entire object,  $\mathcal{T}$  is the time-ordering operator, and

$$H_{\text{total}} = H_S + H_B + H_{SB}, \quad (\text{S4})$$

where  $H_S, H_B, H_{SB}$  are terms in the Hamiltonian that depend only on degrees of freedom of  $S$ ,  $B$ , or both, respectively. Taking the trace of Eq. S3 with respect to the states of  $B$  yields

$$\rho(T) = \sum_{\alpha\beta} p_{\beta} E_{\alpha\beta}(T) \rho(0) E_{\alpha\beta}^{\dagger}(T) \quad (\text{S5})$$

where

$$E_{\alpha\beta}(T) = \langle e_{\alpha} | U(T) | e_{\beta} \rangle, \quad (\text{S6})$$

is a Kraus operator and Eq. (S5) is known as the *operator sum representation* [1, 2].

By identifying:

$$\begin{aligned} \chi_{abcd}(T) &= \sum_{\alpha\beta} [E_{\alpha\beta}(t)]_{ac} [E_{\alpha\beta}^{\dagger}(t)]_{db} \\ &= \sum_{\alpha\beta} p_{\beta} \langle e_{\alpha}, a | U(T) | e_{\beta}, c \rangle \langle e_{\beta}, d | U^{\dagger}(T) | e_{\alpha}, b \rangle \end{aligned} \quad (\text{S7})$$

we have proven the equivalence between Eq. S5 and 1 in the article. An important caveat which is clear from the derivation is the following:  $\rho_B(0)$  must be the same for every initial state in  $S$  for  $\chi(T)$  to be well-defined. Also, different states  $\rho_B(0)$  will obviously yield different processes.

□

PROOF OF EQ. 2 IN THE ARTICLE.— Manipulating Eq. S7, it follows that

$$\begin{aligned}
\chi_{badc}(T) &= \sum_{\alpha\beta} p_\beta \langle e_\alpha, b | U(T) | e_\beta, d \rangle \langle e_\beta, c | U^\dagger(T) | e_\alpha, a \rangle \\
&= \left( \sum_{\alpha\beta} p_\beta \langle e_\alpha, a | U(T) | e_\beta, c \rangle \langle e_\beta, d | U^\dagger(T) | e_\alpha, b \rangle \right)^* \\
&= \chi_{abcd}^*(T).
\end{aligned} \tag{S8}$$

□

Eq. 2 in the article preserves the Hermiticity of the density matrix.

$$\begin{aligned}
\rho_{ba}(T) &= \sum_{cd} \chi_{badc}(T) \rho_{dc}(0) \\
&= \sum_{cd} \chi_{abcd}^*(T) \rho_{cd}^*(0) \\
&= \left[ \sum_{cd} \chi_{abcd}(T) \rho_{cd}(0) \right]^* \\
&= \rho_{ab}^*(T).
\end{aligned} \tag{S9}$$

PROOF OF EQ. 3 IN THE ARTICLE.— Using Eq. S7, and exploiting the fact that  $U(T)U^\dagger(T) = U^\dagger(T)U(T) = I_S \otimes I_B$ , the identity on the whole space, we get:

$$\begin{aligned}
\sum_a \chi_{aacd}(T) &= \sum_{a\alpha\beta} p_\beta \langle e_\alpha, a | U(T) | e_\beta, c \rangle \langle e_\beta, d | U^\dagger(T) | e_\alpha, a \rangle \\
&= \sum_{a\alpha\beta} p_\beta \langle e_\beta, d | U^\dagger(T) | e_\alpha, a \rangle \langle e_\alpha, a | U(T) | e_\beta, c \rangle \\
&= \sum_{\beta} p_\beta \langle e_\beta, d | e_\beta, c \rangle \\
&= \delta_{cd}.
\end{aligned} \tag{S10}$$

□

Eq. 3 in the article preserves the trace of the density matrix:

$$\begin{aligned}
\text{Tr}(\rho(T)) &= \sum_{acd} \chi_{aacd}(T) \rho_{cd}(0) \\
&= \sum_{cd} \delta_{cd} \rho_{cd}(0) \\
&= \text{Tr}(\rho(0)).
\end{aligned} \tag{S11}$$

PROOF OF EQ. 4 IN THE ARTICLE.— Again, manipulating Eq. S7:

$$\begin{aligned}
\sum_{abcd} z_{ac}^* \chi_{abcd}(T) z_{bd} &= \sum_{abcd} z_{ac}^* \sum_{\alpha\beta} p_\beta \langle e_\alpha, a | U(T) | e_\beta, c \rangle \langle e_\beta, d | U^\dagger(T) | e_\alpha, b \rangle z_{bd} \\
&= \sum_{\alpha\beta} p_\beta \zeta_\alpha \zeta_\alpha^* \\
&\geq 0,
\end{aligned}$$

where we have defined  $\zeta_\alpha = \sum_{ac} z_{ac}^* \langle e_\alpha, a | U(T) | e_\beta, c \rangle$ .  $\square$ .

Suppose  $\rho(0)$  is Hermitian positive-semidefinite (HPS), so that we may write  $\rho_{cd}(0) = \sum_k U_{kc}^* q_k U_{kd}$  where  $U$  is a unitary transformation that diagonalizes  $\rho(0)$ , and  $q_k \geq 0$  for all  $k$ . Is the HPS condition maintained for  $\rho(T)$ ? If so, it must satisfy  $\sum_{ab} y_a^* \rho_{ab}(T) y_b \geq 0$  for an arbitrary vector  $y$ . Eq. 4 in the article guarantees this:

$$\begin{aligned}
\sum_{ab} y_a^* \rho_{ab}(T) y_b &= \sum_{abcdk} y_a^* \chi_{abcd}(T) U_{kc}^* q_k U_{kd} y_b \\
&= \sum_k \sum_{abcd} z_{ac}^{(k)*} \chi_{abcd}(T) z_{bd}^{(k)} \\
&\geq 0,
\end{aligned}$$

where we have identified the vectors  $z^{(k)}$  with elements  $z_{bd}^{(k)} = \sqrt{q_k} U_{kd} y_b$ .

## II. TRANSITION DIPOLES OF THE COUPLED DIMER MODEL

Since we are concerned with the interaction of the chromophores with electromagnetic radiation, we make some remarks on the geometry of the transition dipoles (see Fig. S1). Let the independent site transition dipole moments from the ground to the single exciton be  $\mathbf{d}_A$  and  $\mathbf{d}_B$ , respectively. The transition dipole moments for the relevant eigenstate transitions are (see for example, [3]):

$$\begin{aligned}
\begin{bmatrix} \boldsymbol{\mu}_{\alpha g} \\ \boldsymbol{\mu}_{\beta g} \end{bmatrix} &= \begin{bmatrix} \cos \theta & \sin \theta \\ -\sin \theta & \cos \theta \end{bmatrix} \begin{bmatrix} \mathbf{d}_A \\ \mathbf{d}_B \end{bmatrix} \\
\begin{bmatrix} \boldsymbol{\mu}_{f\alpha} \\ \boldsymbol{\mu}_{f\beta} \end{bmatrix} &= \begin{bmatrix} \sin \theta & \cos \theta \\ \cos \theta & -\sin \theta \end{bmatrix} \begin{bmatrix} \mathbf{d}_A \\ \mathbf{d}_B \end{bmatrix}.
\end{aligned} \tag{S12}$$

To simplify notation, we assume that  $J \neq 0$  and the components of  $\mathbf{d}_A$  and  $\mathbf{d}_B$  are all real, which imply that  $\boldsymbol{\mu}_{ij} = \boldsymbol{\mu}_{ji}$ , for all  $i, j \in \{\alpha, \beta, f\}$ . For a coupled heterodimer, the four dipoles in Eq. (S12) are located in the same plane, but in general have different magnitudes

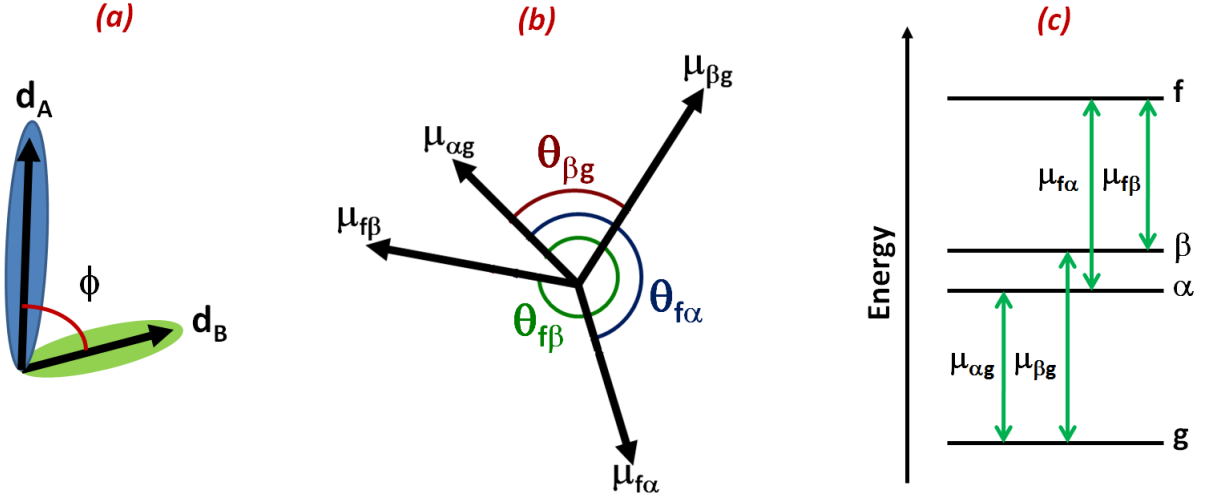

Figure S1: *Parameters of the coupled heterodimer.* (a) Dipole vectors  $\mathbf{d}_A$  and  $\mathbf{d}_B$  for each chromophoric site. The angle between them is  $\phi$ . (b) Transition dipole moments between the different eigenstates of  $H_S$ ; angles are referenced with respect to  $\mu_{\alpha g}$ . (c) Energy spectrum of  $H_S$  and allowed dipole transitions.

and directions. We label the magnitude of  $\mu_{ij}$  with  $\mu_{ij}$  and the angle between  $\mu_{ij}$  and  $\mu_{\alpha g}$  with  $\phi_{ij}$ , so that the reference is with respect to  $\theta_{\alpha g} = 0$  (Fig. S1).

The different transition dipole moments can be easily expressed in terms of the angle  $\phi$  between  $\mathbf{d}_A$  and  $\mathbf{d}_B$ , and the mixing angle  $\theta$ . We present these functional dependences for completeness. We define our coordinate axes so

$$\begin{aligned}\mathbf{d}_A &= d_A \hat{z}, \\ \mathbf{d}_B &= (d_B \cos \phi) \hat{z} + (d_B \sin \phi) \hat{x}.\end{aligned}\tag{S13}$$

We can express the components of the transition dipole moments,

$$\begin{aligned}\mu_{\alpha g} &= (d_B \sin \theta \sin \phi) \hat{x} + (d_A \cos \theta + d_B \sin \theta \cos \phi) \hat{z}, \\ \mu_{\beta g} &= (d_B \cos \theta \sin \phi) \hat{x} + (-d_A \sin \theta + d_B \cos \theta \cos \phi) \hat{z}, \\ \mu_{f\alpha} &= (d_B \cos \theta \sin \phi) \hat{x} + (d_A \sin \theta + d_B \cos \theta \cos \phi) \hat{z}, \\ \mu_{f\beta} &= (-d_B \sin \theta \sin \phi) \hat{x} + (d_A \cos \theta - d_B \sin \theta \cos \phi) \hat{z}.\end{aligned}\tag{S14}$$

The angles between the different transition dipole moments can be calculated as

$$\begin{aligned}\cos(\phi_{ij}) &= \frac{\mu_{\alpha g} \cdot \mu_{ij}}{\mu_{\alpha g} \mu_{ij}}, \\ \sin(\phi_{ij}) &= \frac{|\mu_{\alpha g} \times \mu_{ij}|}{\mu_{\alpha g} \mu_{ij}}.\end{aligned}\tag{S15}$$



where  $\mu_{ij}$  denotes the norm of the respective dipole. For a homodimer with  $\theta = \frac{\pi}{4}$ ,  $d_A = d_B$  and  $\boldsymbol{\mu}_{f\alpha} = \boldsymbol{\mu}_{\alpha g}$ ,  $\boldsymbol{\mu}_{f\beta} = -\boldsymbol{\mu}_{\beta g}$ , yielding only two independent directions for the four transition dipoles [4]. For a homodimer with  $\theta = \frac{3\pi}{4}$ , the conclusion is similar.

### III. STATE PREPARATION. DERIVATION OF EQUATION (9) IN THE ARTICLE

The second order density matrix in  $\lambda$  that results after considering the components of the first two pulses at  $-\mathbf{k}_1$  and  $+\mathbf{k}_2$  can be calculated in Liouville space as (see [5]),

$$\begin{aligned} & \tilde{\rho}_{\mathbf{e}_1, \mathbf{e}_2}^{\omega_1, \omega_2}(t_2 + T) \\ &= \left(\frac{1}{i}\right)^2 \int_{-\infty}^{t_2+T} dt'' \int_{-\infty}^{t''} dt' \mathcal{G}_2(t_2 + T, t'') \tilde{\mathcal{V}}(t'') \mathcal{G}_1(t'', t') \tilde{\mathcal{V}}(t') \rho(-\infty), \end{aligned} \quad (\text{S16})$$

where  $\rho(-\infty) = |g\rangle\langle g|$ , or alternatively, in Liouville space notation,  $\rho(-\infty) = |gg\rangle\rangle$ , is the state of the system before the perturbations. We are interested in the situation  $T > 3\sigma$ , that is, after the action of the two pulses has practically ceased. The perturbation superoperator is  $\tilde{\mathcal{V}}(t) = \sum_{i=1}^3 \tilde{\mathcal{V}}_i(t)$ , where  $\tilde{\mathcal{V}}_i(t) = [\tilde{V}_i, \cdot]$ , and

$$\begin{aligned} \tilde{V}_1(t) &= -\lambda \hat{\boldsymbol{\mu}}^< \cdot \mathbf{e}_1 E(t - t_1) e^{i\omega_1(t-t_1)} \\ \tilde{V}_2(t) &= -\lambda \hat{\boldsymbol{\mu}}^> \cdot \mathbf{e}_2 E(t - t_2) e^{-i\omega_2(t-t_2)} \\ \tilde{V}_3(t) &= -\lambda \hat{\boldsymbol{\mu}}^> \cdot \mathbf{e}_3 E(t - t_3) e^{-i\omega_3(t-t_3)}. \end{aligned} \quad (\text{S17})$$

These expressions conveniently adapt Eq. 6 in the article to account for the phase matching direction of  $\mathbf{k}_{PE}$  and to consider the RWA, where  $\hat{\boldsymbol{\mu}}^< = \sum_{\omega_p < \omega_q} \boldsymbol{\mu}_{pq} |p\rangle\langle q|$  promotes emissions from the ket or absorptions on the bra, and  $\hat{\boldsymbol{\mu}}^> = (\hat{\boldsymbol{\mu}}^<)^+$  induces the opposite processes.

#### A. Well separated pulses 1 and 2

We can simplify Eq. S16 by considering that: (a) if  $\tau > 3\sigma$ , the pulses are well separated, and we can perform the substitution  $\tilde{\mathcal{V}}(t') = \tilde{\mathcal{V}}_1(t')$  and  $\tilde{\mathcal{V}}(t'') = \tilde{\mathcal{V}}_2(t'')$ ; (b) we focus only on the dominant contribution due to the resonant transitions. As mentioned in the text, this calculation can be easily grasped by analyzing the double-sided Feynman diagrams in Fig. 2a–d. Since we are looking for signals only in the direction  $-\mathbf{k}_1 + \mathbf{k}_2 + \mathbf{k}_3$ , the first pulse must interact via the operator  $\hat{\boldsymbol{\mu}}^<$ , so it can only act on the bra to produce optical coherences  $|gp\rangle\rangle$ . We assume that these coherences evolve unitarily together with a constant dephasing rate (this assumption is not necessary, but it simplifies our analysis):

$$\begin{aligned} \mathcal{G}_1(t'', t') &= \mathcal{G}(t'' - t') \\ &= \sum_{mn} \mathcal{G}_{mn}(t'' - t') |mn\rangle\rangle\langle\langle mn|, \end{aligned} \quad (\text{S18})$$

where  $\mathcal{G}_{mn}(\tau)$  is given by Eq. 11 in the article. The second pulse can act on the ket to create the coherence  $|pq\rangle\rangle$  if  $p \neq q$ . However, in case the frequency component of the second pulse is the same as that of the first pulse, it can excite the ket to form a population  $|qq\rangle\rangle$  or de-excite the bra to go back to  $-|gg\rangle\rangle$  (with opposite sign due to the commutator). For the evolution in the waiting time, we use the following identity:

$$\mathcal{G}_2(t_2 + T, t'') = \chi(T)\mathcal{G}(t_2 - t''), \quad (\text{S19})$$

where we have formally introduced the process matrix  $\chi(T)$  acting as the propagator after time  $t_2$ . Altogether, we have in Liouville space a perturbation, a free evolution, another perturbation, and free evolution. The effective second order density matrix associated with the perturbations at  $-\mathbf{k}_1 + \mathbf{k}_2$  is given by:

$$\begin{aligned} & \tilde{\rho}_{\mathbf{e}_1, \mathbf{e}_2}^{\omega_1, \omega_2}(t_2 + T) \\ &= - \left( \frac{-\lambda}{i} \right)^2 \sum_{pq} \left[ \int_{-\infty}^{t_2+T} dt'' \chi(T) \left\{ \mathcal{G}_{qp}(t_2 - t'') \left( \boldsymbol{\mu}_{qg} \cdot \mathbf{e}_2 |q\rangle\langle g| E(t'' - t_2) e^{-i\omega_2(t'' - t_2)} \right) \right. \right. \\ & \quad \times \int_{-\infty}^{t''} dt' \mathcal{G}_{gp}(t'' - t') |g\rangle\langle g| \left( |g\rangle\langle p| \boldsymbol{\mu}_{pg} \cdot \mathbf{e}_1 E(t' - t_1) e^{i\omega_1(t' - t_1)} \right) \Big\} \\ & \quad - \int_{-\infty}^{t_2+T} dt'' \chi(T) \left\{ \mathcal{G}_{gg}(t_2 - t'') \right. \\ & \quad \times \int_{-\infty}^{t''} dt' \mathcal{G}_{gp}(t'' - t') |g\rangle\langle g| \left( |g\rangle\langle p| \boldsymbol{\mu}_{pg} \cdot \mathbf{e}_1 E(t' - t_1) e^{i\omega_1(t' - t_1)} \right) \\ & \quad \times \left. \left( |q\rangle\langle g| \boldsymbol{\mu}_{qg} \cdot \mathbf{e}_2 E(t'' - t_2) e^{i\omega_1(t'' - t_2)} \right) \right\} \Big] \end{aligned} \quad (\text{S20})$$

This calculation is a double integral over all the possible times  $t'$  and  $t''$  in which the perturbations due to the pulses at  $-\mathbf{k}_1$  and  $+\mathbf{k}_2$  can act due to their finite width  $\sigma$ . The time-ordering consideration is unimportant for  $\tau, T \gg \sigma$ , and in fact, both integrals can be extended to the entire real space:  $\int_{-\infty}^{t_2+T} dt'' \int_{-\infty}^{t''} dt'(\cdot) \approx \int_{-\infty}^{\infty} dt'' \int_{-\infty}^{\infty} dt'(\cdot)$ . As discussed in the next subsection, the approximation  $T \gg \sigma$  is needed (so that the pulse envelopes are nearly zero at time  $t_2 + T$ ), but the  $\tau \gg \sigma$  assumption is unnecessary. We then rewrite

$$\begin{aligned} & \approx - \left( \frac{-\lambda}{i} \right)^2 \sum_{pq} (\boldsymbol{\mu}_{pg} \cdot \mathbf{e}_1) (\boldsymbol{\mu}_{qg} \cdot \mathbf{e}_2) \\ & \quad \times \int_{-\infty}^{\infty} d(t' - t_1) \left( \mathcal{G}_{gp}(t_1 - t') E(t' - t_1) e^{i\omega_1(t' - t_1)} \right) \\ & \quad \times \chi(T) \left\{ \int_{-\infty}^{\infty} d(t_2 - t'') \mathcal{G}_{qp}(t_2 - t'') E(t'' - t_2) e^{-i\omega_2(t'' - t_2)} \mathcal{G}_{gp}(t'' - t_2) |q\rangle\langle p| \right. \\ & \quad \left. - \delta_{pq} (\mathcal{G}_{gg}(t_2 - t'') E(t'' - t_2) e^{-i\omega_2(t'' - t_2)} \mathcal{G}_{gp}(t'' - t_2) |g\rangle\langle g|) \right\} \end{aligned} \quad (\text{S21})$$

The length of the pulse  $\sigma$  is much shorter than the dynamics induced by the bath. Therefore,  $\sigma \ll \frac{1}{\Gamma_{mn}}$ , and dephasing contributions can be neglected within the integral so that  $\mathcal{G}_{gp}(t_1 - t') \approx e^{i\omega_{pg}(t_1 - t')}$ ,  $\mathcal{G}_{qp}(t_2 - t'')\mathcal{G}_{gp}(t'' - t_2) \approx e^{-i\omega_{qp}(t_2 - t'')}e^{i\omega_{pg}(t_2 - t'')} = e^{-i\omega_{qg}(t_2 - t'')}$ , and  $\mathcal{G}_{gp}(t'' - t_2) \approx e^{-i\omega_{pg}(t'' - t_2)}$ ,  $\mathcal{G}_{gg}(t'' - t_2) \approx e^{-i\omega_{gg}(t'' - t_2)}$ . However, the dephasing terms are non-negligible in the free evolution between the pulses if  $\tau \gg \sigma$ , and the term  $\mathcal{G}_{gp}(\tau)$  in the final expression cannot in general be simplified to  $e^{-i\omega_{gp}\tau}$ . Then we have

$$\begin{aligned} & \approx -\left(\frac{-\lambda}{i}\right)^2 \sum_{pq} (\boldsymbol{\mu}_{pg} \cdot \mathbf{e}_1)(\boldsymbol{\mu}_{qg} \cdot \mathbf{e}_2) \int_{-\infty}^{\infty} ds' e^{-i\omega_{pg}s'} E(s') e^{i\omega_1 s'} \int_{-\infty}^{\infty} ds'' e^{i\omega_{pg}s''} \\ & \quad \times \chi(T) \left\{ E(s'') e^{-i\omega_2 s''} (|q\rangle\langle p| - \delta_{pq}|g\rangle\langle g|) \right\} \\ & = -\chi(T) \left\{ \sum_{pq} C_{\omega_1}^p C_{\omega_2}^q (\boldsymbol{\mu}_{pg} \cdot \mathbf{e}_1)(\boldsymbol{\mu}_{qg} \cdot \mathbf{e}_2) \mathcal{G}_{gp}(t_2 - t_1) (|q\rangle\langle p| - \delta_{pq}|g\rangle\langle g|) \right\}, \quad (\text{S22}) \end{aligned}$$

The final result has a clear physical interpretation: Each of the transitions depicted in the diagrams in Fig. 2a-d is controlled by the frequency components of the pulse at the given transition (terms  $C_{\omega_1}^p$  and  $C_{\omega_2}^q$ ), as well as the alignment between the transition dipole and the pulse polarization. Free evolution of the optical coherence between the perturbations is given by  $\mathcal{G}_{gp}(\tau)$ . Once the state  $|q\rangle\langle p| - \delta_{pq}|g\rangle\langle g|$  is formed, the superoperator  $\chi(T)$  acts on it, encoding both coherent and dissipative processes.

## B. Overlapping pulses 1 and 2

We now consider  $0 \leq \tau < 3\sigma$ . Eq. (9) in the article rigorously holds for this more general case. For the contribution due to the original diagrams in Fig. 2a-d, we carry out the same double integral of Eq. (S20), but we keep it time ordered as  $\int_{-\infty}^{\infty} dt'' \int_{-\infty}^{t''} dt'(\cdot)$ . Additionally, each diagram in Fig. 2a-d corresponds to another diagram where the pulse at  $+\mathbf{k}_2$  acts before the one at  $-\mathbf{k}_1$ , but yields back the same state after the two pulses (for example, the one corresponding to Fig. 2b would be  $gg \rightarrow \beta g \rightarrow \beta\alpha$ ). Their contributions to  $[\rho_{-\mathbf{k}_1, \mathbf{k}_2}^{(2)}]_{\mathbf{e}_1, \mathbf{e}_2}^{\omega_1, \omega_2}(t_2 + T)$  can be easily shown to be  $\int_{-\infty}^{\infty} dt'' \int_{t''}^{\infty} dt'(\cdot)$ , where the integrand and the dummy variable convention are the same as before. The sum of the two contributions yields back the double integral as in Eq. (S21).

## IV. STATE DETECTION. DERIVATION OF EQUATIONS 14-16 IN THE ARTICLE

The techniques to derive these equations are the same as the ones used for the previous section. However, the proliferation of terms makes the full exposition of the derivation unwieldy. Therefore, we only illustrate how some sample terms arise.

### A. Well separated pulses 3 and 4

Let us start by noting that, using Eq. (9) in the article, the element  $ij$  of  $\tilde{\rho}_{\mathbf{e}_1, \mathbf{e}_2}^{\omega_1, \omega_2}(t_2 + T)$  can be expressed as:

$$\begin{aligned} & \langle i | \tilde{\rho}_{\mathbf{e}_1, \mathbf{e}_2}^{\omega_1, \omega_2}(t_2 + T) | j \rangle \\ & \left\langle i \left| -\chi(T) \left\{ \sum_{pq} C_{\omega_1}^p C_{\omega_2}^q (\boldsymbol{\mu}_{pg} \cdot \mathbf{e}_1) (\boldsymbol{\mu}_{qg} \cdot \mathbf{e}_2) \mathcal{G}_{gp}(\tau) (|q\rangle\langle p| - \delta_{pq} |g\rangle\langle g|) \right\} \right| j \right\rangle \\ & = - \sum_{pq} C_{\omega_1}^p C_{\omega_2}^q (\boldsymbol{\mu}_{pg} \cdot \mathbf{e}_1) (\boldsymbol{\mu}_{qg} \cdot \mathbf{e}_2) \mathcal{G}_{gp}(\tau) (\chi_{ijqp}(T) - \delta_{pq} \delta_{ij} \delta_{ig}). \end{aligned} \quad (\text{S23})$$

We define  $[\rho_{-\mathbf{k}_1, \mathbf{k}_2, \mathbf{k}_3}^{(3)}]_{\mathbf{e}_1, \mathbf{e}_2, \mathbf{e}_3}^{\omega_1, \omega_2, \omega_3}(t_3 + t)$  analogously to the way  $\tilde{\rho}_{\mathbf{e}_1, \mathbf{e}_2}^{\omega_1, \omega_2}(t_2 + T)$  was defined in Eq. (S16), that is, the third-order in  $\lambda$  density matrix due to the perturbations corresponding to the phase-matching direction  $-\mathbf{k}_1 + \mathbf{k}_2 + \mathbf{k}_3$ . For  $t \gg \sigma$ , we can easily calculate the matrix elements of  $[\rho_{-\mathbf{k}_1, \mathbf{k}_2, \mathbf{k}_3}^{(3)}]_{\mathbf{e}_1, \mathbf{e}_2, \mathbf{e}_3}^{\omega_1, \omega_2, \omega_3}(t_3 + t)$  that yield an optical dipole, say  $\alpha g$ , and can then find the contribution of the latter to the polarization via trace with respect to  $\hat{\boldsymbol{\mu}}$  (see Fig. 2e and h):

$$\begin{aligned} & \text{Tr}(\hat{\boldsymbol{\mu}} \langle \alpha | [\rho_{-\mathbf{k}_1, \mathbf{k}_2, \mathbf{k}_3}^{(3)}]_{\mathbf{e}_1, \mathbf{e}_2, \mathbf{e}_3}^{\omega_1, \omega_2, \omega_3}(t_3 + t) | g \rangle | \alpha \rangle \langle g |) \\ & = - \text{Tr}[\hat{\boldsymbol{\mu}} \sum_{pq} C_{\omega_1}^p C_{\omega_2}^q (\boldsymbol{\mu}_{pg} \cdot \mathbf{e}_1) (\boldsymbol{\mu}_{qg} \cdot \mathbf{e}_2) \mathcal{G}_{gp}(\tau) \\ & \quad \times \left( \frac{-\lambda}{i} \right) \int_{-\infty}^{t_3+t} dt' \mathcal{G}_{\alpha g}(t_3 + t - t') E(t' - t_3) e^{-i\omega_3(t' - t_3)} \\ & \quad \times \{ (\boldsymbol{\mu}_{\alpha g} \cdot \mathbf{e}_3 | \alpha \rangle \langle g |) (e^{-i\omega_{gg}(t' - t_3)} (\chi_{ggqp}(T) - \delta_{pq}) | g \rangle \langle g |) \\ & \quad - (e^{-i\omega_{\alpha\alpha}(t' - t_3)} \chi_{\alpha\alpha qp}(T) | \alpha \rangle \langle \alpha |) (| \alpha \rangle \langle g | \boldsymbol{\mu}_{\alpha g} \cdot \mathbf{e}_3) \\ & \quad - (e^{-i\omega_{\alpha\beta}(t' - t_3)} \chi_{\alpha\beta qp}(T) | \alpha \rangle \langle \beta |) (| \beta \rangle \langle g | \boldsymbol{\mu}_{\beta g} \cdot \mathbf{e}_3) \} \\ & \approx - \sum_{pq} C_{\omega_1}^p C_{\omega_2}^q (\boldsymbol{\mu}_{pg} \cdot \mathbf{e}_1) (\boldsymbol{\mu}_{qg} \cdot \mathbf{e}_2) \mathcal{G}_{gp}(\tau) \\ & \quad \times \{ C_{\omega_3}^{\alpha} (\boldsymbol{\mu}_{\alpha g} \cdot \mathbf{e}_3) \mathcal{G}_{\alpha g}(t) (\chi_{ggqp}(T) - \delta_{pq} - \chi_{\alpha\alpha qp}(T)) \\ & \quad - C_{\omega_3}^{\beta} (\boldsymbol{\mu}_{\beta g} \cdot \mathbf{e}_3) \mathcal{G}_{\alpha g}(t) \chi_{\alpha\beta qp}(T) \} \boldsymbol{\mu}_{\alpha g}, \end{aligned} \quad (\text{S24})$$

where, just as before, we have used the fact that  $\sigma \ll \frac{1}{\Gamma_{\alpha g}}$  to approximate that  $\mathcal{G}_{\alpha g}(t_3 + t - t') \approx \mathcal{G}_{\alpha g}(t) e^{i\omega_{\alpha g}(t' - t_3)}$ , and the integrals have been extended to the entire real axis. The third pulse at  $+\mathbf{k}_3$  can excite the ket or de-excite the bra of the output state at the waiting time. The calculation above simply enumerates the resonant transitions  $gg, \alpha\alpha, \alpha\beta \rightarrow \alpha g$  due to the laser components associated with  $C_{\omega_3}^{\alpha}$ ,  $C_{\omega_3}^{\alpha}$ , and  $C_{\omega_3}^{\beta}$ , respectively, and takes the trace of the optical coherence with respect to the dipole operator:  $\text{Tr}(\hat{\boldsymbol{\mu}} | \alpha \rangle \langle g |) = \boldsymbol{\mu}_{\alpha g}$ . Recall that we have chosen the dipole elements to be purely real.

The detection of the polarization due to the  $\alpha g$  coherence occurs through heterodyning. The fourth ultrashort pulse interferes with the coherence oscillating as  $e^{i\omega_{\alpha g}(t''-t_4)}$ , yielding a contribution to the time integrated signal encoded by:

$$\begin{aligned} & \int_{-\infty}^{\infty} dt'' e^{i\omega_4(t''-t_4)} E(t''-t_4) e^{-i\omega_{\alpha g}(t''-t_4)} \\ &= i\sqrt{2\pi\sigma^2} e^{-\sigma^2(\omega_{\alpha g}-\omega_4)^2/2} \\ &\propto C_{\omega_4}^{\alpha}. \end{aligned} \quad (\text{S25})$$

In words, the Fourier components of the fourth pulse filter the optical coherences of the polarization associated sample. In our case, the polarization due to the coherence  $\alpha g$  will be detected as  $C_{\omega_4}^{\alpha}$ , that is, proportionally to the frequency component of the fourth pulse at  $\omega_{\alpha g}$ . Altogether, the calculation reads:

$$\begin{aligned} & \int_{-\infty}^{\infty} e^{i\omega_4(t''-t_4)} E(t''-t_4) e^{-i\omega_{\alpha g}(t''-t_4)} \\ & \times \mathbf{e}_4 \cdot \text{Tr}(\hat{\boldsymbol{\mu}} \langle \alpha | [\rho_{-\mathbf{k}_1, \mathbf{k}_2, \mathbf{k}_3}^{(3)}]_{\mathbf{e}_1, \mathbf{e}_2, \mathbf{e}_3}^{\omega_1, \omega_2, \omega_3}(t_3+t) | g \rangle | \alpha \rangle \langle g |) \\ & \propto C_{\omega_4}^{\alpha} \mathbf{e}_4 \cdot \text{Tr}(\hat{\boldsymbol{\mu}} \langle \alpha | [\rho_{-\mathbf{k}_1, \mathbf{k}_2, \mathbf{k}_3}^{(3)}]_{\mathbf{e}_1, \mathbf{e}_2, \mathbf{e}_3}^{\omega_1, \omega_2, \omega_3}(t_3+t) | g \rangle | \alpha \rangle \langle g |) \\ &= - \sum_{pq} C_{\omega_1}^p C_{\omega_2}^q (\boldsymbol{\mu}_{pg} \cdot \mathbf{e}_1) (\boldsymbol{\mu}_{qg} \cdot \mathbf{e}_2) \mathcal{G}_{gp}(\tau) \\ & \times \{ C_{\omega_3}^{\alpha} C_{\omega_4}^{\alpha} (\boldsymbol{\mu}_{\alpha g} \cdot \mathbf{e}_3) (\boldsymbol{\mu}_{\alpha g} \cdot \mathbf{e}_4) \mathcal{G}_{\alpha g}(t) (\chi_{ggqp}(T) - \delta_{pq} - \chi_{\alpha\alpha qp}(T)) \\ & - C_{\omega_3}^{\beta} C_{\omega_4}^{\alpha} (\boldsymbol{\mu}_{\beta g} \cdot \mathbf{e}_3) (\boldsymbol{\mu}_{\alpha g} \cdot \mathbf{e}_4) \mathcal{G}_{\alpha g}(t) \chi_{\alpha\beta qp}(T) \}. \end{aligned} \quad (\text{S26})$$

This exercise can be repeated for the rest of the optical coherences which occur in the echo time and yield detectable dipoles:  $\beta g, f\alpha, f\beta$  (Fig. 2-e,f,g,h). The total signal is

$$\begin{aligned} & [S_{PE}]_{\mathbf{e}_1, \mathbf{e}_2, \mathbf{e}_3, \mathbf{e}_4}^{\omega_1, \omega_2, \omega_3, \omega_4}(\tau, T, t) \\ &= \sum_{uv=\alpha g, \beta g, f\alpha, f\beta} \int_{-\infty}^{\infty} dt'' e^{i\omega_4(t''-t_4)} E(t''-t_4) e^{-i\omega_{ij}(t''-t_4)} \\ & \times \mathbf{e}_4 \cdot \text{Tr}(\hat{\boldsymbol{\mu}} \langle u | [\rho_{-\mathbf{k}_1, \mathbf{k}_2, \mathbf{k}_3}^{(3)}]_{\mathbf{e}_1, \mathbf{e}_2, \mathbf{e}_3}^{\omega_1, \omega_2, \omega_3}(t_3+t) | v \rangle | u \rangle \langle v |), \end{aligned} \quad (\text{S27})$$

which yields Eq. 14 in the article. That equation has been rewritten by grouping the terms in the forms of Eqs. 15 and 16 in the article, and their analogues upon the  $\alpha, \beta \rightarrow \beta, \alpha$  substitutions in order to classify the processes corresponding to the frequencies of the transition due to the third pulse and the heterodyne detection.

## B. Overlapping pulses 3 and 4

We now consider  $0 \leq t$  rather than  $3\sigma < t$ , to consider overlapping pulses 3 and 4. Eq. 14 in the article must be slightly modified when the overlap in time between the third and the fourth pulses is significant. As opposed to Section III-B of this Appendix, where the first pulse can act on the system before the second pulse *and* viceversa, in the detection stage, the third pulse must act on the system to yield a polarization *before* the fourth pulse (which does not interact with the system) can detect it. Hence, the LO cannot be regarded on the same footing as the other three pulses.

First, we state the solution to the relevant integral:

$$\begin{aligned} & \int_{-\infty}^{\infty} dt'' \int_{-\infty}^{t''} dt' e^{i\omega_4(t''-t_4)} E(t''-t_4) e^{-i\omega_{uv}(t''-t_4)} \mathcal{G}_{uv}(t) e^{i\omega_{uv}(t'-t_3)} E(t'-t_3) e^{-i\omega_3(t'-t_3)} e^{-i\omega_{ij}(t'-t_3)} \\ &= \left( \sqrt{\pi\sigma^2} e^{-(\omega_3 - (\omega_{uv} - \omega_{ij}))^2 \sigma^2 / 2} \right) \left( \sqrt{\pi\sigma^2} e^{-(\omega_4 - (\omega_4 - \omega_{uv}))^2} \right) \\ & \times \left( 1 + \text{Erf} \left( \frac{t}{2\sigma} + \frac{(\omega_3 - (\omega_{uv} - \omega_{ij}) + \omega_4 - \omega_{uv})\sigma}{2} \right) \right) \mathcal{G}_{uv}(t), \end{aligned} \quad (\text{S28})$$

which applies to the  $ij \rightarrow uv$  transition caused by the third pulse at  $+k_3$ , followed by an effective free evolution  $\mathcal{G}_{uv}(t)$  for the echo interval  $t = t_4 - t_3$ , and the detection of the optical coherence  $uv$  via the LO. Importantly, the upper limit of the integral over  $t'$ , associated with the action of the third pulse, cannot be taken to  $\infty$ , since the LO may interfere with the transients of the polarization before the envelope of the third pulse is effectively over. There is no contribution from the complementary integral going from  $t''$  to  $\infty$  since the LO is assumed not to interact with the system and, hence, does not contribute to the polarization of the sample.

Repeating the derivation of Eq. S24 by not taking the upper limit of the  $t''$  integral to  $\infty$ , it can be seen that the only modification to Eq. 14 in the article is given by Eq. 17 in the article. That is, the amplitudes of the third transition and the action of the LO are correlated by an error function. In the limiting case when  $t \gg \sigma$ , Eq. 17 recovers  $C_{\omega_3}^r C_{\omega_4}^s$ , since  $\text{Erf}(x) \rightarrow 1$  as  $\Re\{x\} \rightarrow \infty$ .

## V. OVERALL MULTIPLICATIVE CONSTANT

OVERALL MULTIPLICATIVE CONSTANT. Eq. (14) in the article is defined up to a proportionality constant which depends on many factors such as the concentration of the molecules in the experimental sample and the efficiency of the mirrors in the optical setup. This factor may be determined by performing the extraction of  $\chi(T)$  up to that constant, and then normalizing

it by enforcing the trace preservation condition of Eq. 3 in the article to hold for population initial states,  $c = d$ .

## VI. ISOTROPIC AVERAGES

The probed sample is an ensemble of isotropically distributed molecules in solution. The isotropic average  $\langle \cdot \rangle$  for a tetradic  $(\boldsymbol{\mu}_a \cdot \mathbf{e}_1)(\boldsymbol{\mu}_b \cdot \mathbf{e}_2)(\boldsymbol{\mu}_c \cdot \mathbf{e}_3)(\boldsymbol{\mu}_d \cdot \mathbf{e}_4)$  is given by [6]:

$$\begin{aligned} & \langle (\boldsymbol{\mu}_a \cdot \mathbf{e}_1)(\boldsymbol{\mu}_b \cdot \mathbf{e}_2)(\boldsymbol{\mu}_c \cdot \mathbf{e}_3)(\boldsymbol{\mu}_d \cdot \mathbf{e}_4) \rangle_{iso} \\ &= \sum_{m_1 m_2 m_3 m_4} I_{e_1 e_2 e_3 e_4; m_1 m_2 m_3 m_4}^{(4)} \\ & \times [(\boldsymbol{\mu}_a \cdot \mathbf{m}_1)(\boldsymbol{\mu}_b \cdot \mathbf{m}_2)(\boldsymbol{\mu}_c \cdot \mathbf{m}_3)(\boldsymbol{\mu}_d \cdot \mathbf{m}_4)], \end{aligned} \quad (\text{S29})$$

where the isotropically invariant tensor is given by,

$$\begin{aligned} & I_{e_1 e_2 e_3 e_4; m_1 m_2 m_3 m_4}^{(4)} \\ &= \frac{1}{30} [\delta_{e_1 e_2} \delta_{e_3 e_4} \quad \delta_{e_1 e_3} \delta_{e_2 e_4} \quad \delta_{e_1 e_4} \delta_{e_2 e_3}] \\ & \times \begin{bmatrix} 4 & -1 & -1 \\ -1 & 4 & -1 \\ -1 & -1 & 4 \end{bmatrix} \begin{bmatrix} \delta_{m_1 m_2} \delta_{m_3 m_4} \\ \delta_{m_1 m_3} \delta_{m_2 m_4} \\ \delta_{m_1 m_4} \delta_{m_2 m_3} \end{bmatrix}. \end{aligned} \quad (\text{S30})$$

Here,  $\mathbf{e}_i$  and  $\mathbf{m}_i$  are the polarizations of the pulses in the lab and the molecular frame, respectively. The isotropic average consists of a sum of molecular frame products  $[(\boldsymbol{\mu}_a \cdot \mathbf{m}_1)(\boldsymbol{\mu}_b \cdot \mathbf{m}_2)(\boldsymbol{\mu}_c \cdot \mathbf{m}_3)(\boldsymbol{\mu}_d \cdot \mathbf{m}_4)]$  weighted by  $I_{e_1 e_2 e_3 e_4; m_1 m_2 m_3 m_4}^{(4)}$ . Via this procedure, Eq. 14 in the article becomes:

$$\langle [S_{PE}]_{\mathbf{e}_1, \mathbf{e}_2, \mathbf{e}_3, \mathbf{e}_4}^{\omega_1, \omega_2, \omega_3, \omega_4}(\tau, T, t) \rangle_{iso} = \sum_{p, q, r} C_{\omega_1}^p C_{\omega_2}^q C_{\omega_3}^r C_{\omega_4}^s \langle P_{\mathbf{e}_1, \mathbf{e}_2, \mathbf{e}_3, \mathbf{e}_4}^{p, q, r, s}(\tau, T, t) \rangle_{iso}. \quad (\text{S31})$$

Due to the structure of Eq. S30, there are signals which vanish in isotropic conditions even though they are finite otherwise. An interesting consequence of this fact is that QPT is not fully realizable for homodimers, since coherence to population and the reverse processes cannot be detected under isotropic conditions [4].

## VII. ERRORS IN STATE PREPARATION AND DETECTION

Nontrivial bath-induced dynamics during the coherence or echo times could decrease the robustness of the QPT. Such dynamics manifest as deviations from Eq. (11) in the article and

could be diagnosed by analyzing the signal  $[S_{PE}]_{\mathbf{e}_1, \mathbf{e}_2, \mathbf{e}_3, \mathbf{e}_4}^{\omega_1, \omega_2, \omega_3, \omega_4}(\tau, T, t)$  collected as a function of  $\tau$ , with fixed  $T$  and  $t$  values, or alternatively, by varying  $t$  with  $\tau, T$  fixed. A detailed study of this possibility will be presented elsewhere. Similarly, if the bath evolves away from its equilibrium configuration during the coherence time, with dynamics dependent on the excitonic state, then the initial state for QPT will not be well-defined. This problem can be avoided by taking  $\tau = t = 0$  (TD/TB experiments) as described in the article and in the next point.

## VIII. DISCUSSION OF THE FACTORIZABLE CONDITION AT $T = 0$

The factorized initial condition assumption in Eq. S1 requires some further discussion. Does it hold for excitonic systems? At  $t = -\infty$ , we can safely assume that  $\rho_{\text{total}}(t = -\infty) = |g\rangle\langle g| \otimes \rho_{B,eq}$ , where  $\rho_{B,eq}$  is an incoherent ensemble of phonons at thermal equilibrium, and the system state is in the ground electronic state. However, this is not the initial state we are concerned with for a QPT in the single exciton manifold. The state we shall worry about is the one after two pulse perturbations.

First, consider the  $\tau = 0$  case (TB and TD experiments). The discussion in Sections III and IV on overlapping pulses is particularly relevant for this situation. Denote  $[\rho_{\text{total}, -\mathbf{k}_1, \mathbf{k}_2}^{(2)}]_{\mathbf{e}_1, \mathbf{e}_2}^{\omega_1, \omega_2}(t_2 + T)$  the total second order density matrix corresponding to the perturbations at the  $-\mathbf{k}_1$  and  $+\mathbf{k}_2$  directions, such that its trace over the bath yields the object  $\tilde{\rho}_{\mathbf{e}_1, \mathbf{e}_2}^{\omega_1, \omega_2}(t_2 + T)$  defined in Eq. 9 in the article. We are interested in the quasi-impulsive limit of the light-matter interaction, where  $\sigma \ll \frac{1}{\lambda}$ , where  $\sigma$  is the duration of the pulses and  $\lambda$  is the characteristic reorganization energy scale of the bath. As mentioned in the article, in accordance with the Franck-Condon principle, we assume the electronic excitation occurs much faster than any nuclei rearrangement, and  $[\rho_{\text{total}, -\mathbf{k}_1, \mathbf{k}_2}^{(2)}]_{\mathbf{e}_1, \mathbf{e}_2}^{\omega_1, \omega_2}(t_2 + T) \approx \tilde{\rho}_{\mathbf{e}_1, \mathbf{e}_2}^{\omega_1, \omega_2}(t_2 + T) \otimes \rho_{B,eq}$ , so that Eq. S1 holds.

For  $\tau > 0$ , the situation needs to be more carefully analyzed. If  $\tau \ll \frac{1}{\lambda}$ , a similar scenario to the one in the previous paragraph applies (the bath is not given enough time to evolve far away from  $\rho_{B,eq}$ ). Another useful case to consider is  $\tau \gg \frac{1}{\lambda}$ , after which  $B$  relaxes to a stationary or quasi-stationary state  $\rho_{B,stat}$ , which may or may not be equal to  $\rho_{B,eq}$ . In order to preserve the factorizable condition, this state  $\rho_{B,stat}$  must be the same for every electronic population and coherence of interest, so that  $[\rho_{\text{total}, -\mathbf{k}_1, \mathbf{k}_2}^{(2)}]_{\mathbf{e}_1, \mathbf{e}_2}^{\omega_1, \omega_2}(t_2 + T) \approx \tilde{\rho}_{\mathbf{e}_1, \mathbf{e}_2}^{\omega_1, \omega_2}(t_2 + T) \otimes \rho_{B,stat}$ . The simplest example of this situation is a Markovian bath, for which  $B$  relaxes to  $\rho_{B,eq}$  after a timescale on the order of  $\frac{1}{\lambda}$ , which is short compared to the dynamics of the system.

For cases beyond the ones described here, factorizable initial conditions might not apply, and a reexamination of QPT protocols for initially correlated states must be advocated [7–9]. We are currently pursuing this line of research.



In conclusion, in order to get consistent results for QPT, TD/TB seem to be the most promising experiments. The standard PE experiments with finite  $\tau$  provide a QPT if the bath is sufficiently “well-behaved,” as described above.

## IX. TRADING FREQUENCY CONTROL FOR TIME DELAY

Several properties of the pulses can be exploited to selectively manipulate the excitons. These include frequencies [10], polarizations [11–13], and time delays [14–16]. In the article, we have only exploited the former to make a transparent connection between a PE and a QPT experiment. However, the case of polarizations and time delays has also been addressed in our recent work [4]. In this section, we address the use of time delays to substitute frequency control.

Eq. 14 in the article can be rewritten as:

$$[S_{PE}]_{\mathbf{e}_1, \mathbf{e}_2, \mathbf{e}_3, \mathbf{e}_4}^{\omega_1, \omega_2, \omega_3, \omega_4}(\tau, T, t) \propto \sum_{p, q, r, s} C_{\omega_1}^p C_{\omega_2}^q C_{\omega_3}^r C_{\omega_4}^s \mathcal{G}_{gp}(\tau) \mathcal{G}_{sg}(t) P_{\mathbf{e}_1, \mathbf{e}_2, \mathbf{e}_3, \mathbf{e}_4}^{p, q, r, s}(0, T, 0), \quad (\text{S32})$$

For simplicity, we have made the approximations:  $\mathcal{G}_{f\alpha}(t) \approx \mathcal{G}_{\beta g}(t)$  and  $\mathcal{G}_{f\beta}(t) \approx \mathcal{G}_{\alpha g}(t)$ . Notice that in Eq. S32, the frequency  $\omega_{pg}$  appears both in the coherence time propagator  $\mathcal{G}_{gp}(\tau)$  as well as in the frequency amplitude of the first transition  $C_{\omega_1}^p$ . A similar observation follows for  $\omega_{sg}$  in the echo time in  $\mathcal{G}_{sg}(t)$  and  $C_{\omega_4}^s$ . The frequency redundancy in the propagators and the transition amplitudes is the key to understand trading of frequency control for time delays.

Upon the collection of the signal along many values of  $\tau$  and  $t$  for a fixed  $T$ , a double one-sided Fourier transformation yields the 2D-ES [4]:

$$S(\omega_\tau, T, \omega_t) = \int_0^\infty d\tau e^{-i\omega_\tau \tau} \int_0^\infty dt e^{i\omega_t t} [S_{PE}]_{\mathbf{e}_1, \mathbf{e}_2, \mathbf{e}_3, \mathbf{e}_4}^{\omega_1, \omega_2, \omega_3, \omega_4}(\tau, T, t) \quad (\text{S33})$$

$$\propto \sum_{p, s=\alpha, \beta} l_{\tau, p}(\omega_\tau) l_{t, s}(\omega_t) S_{ps}(T) \quad (\text{S34})$$

The spectrum consists of a sum of four resonances at  $(\omega_\tau, \omega_t) \in \{(\omega_{\alpha g}, \omega_{\alpha g}), (\omega_{\alpha g}, \omega_{\beta g}), (\omega_{\beta g}, \omega_{\alpha g}), (\omega_{\beta g}, \omega_{\beta g})\}$ , which correspond to the frequencies of the optical coherences at the coherence and echo times. These resonances are modulated by lineshape functions of the form,

$$l_{\tau, p}(\omega_\tau) = \frac{1}{i(\omega_\tau - \omega_{pg} - i\Gamma_{pg})}, \quad (\text{S35})$$

$$l_{t, s}(\omega_t) = \frac{1}{i(-\omega_t + \omega_{sg} - i\Gamma_{sg})}, \quad (\text{S36})$$

and the amplitude of each peak is given by

$$S_{ps}(T) = \sum_{q, r} C_{\omega_1}^p C_{\omega_2}^q C_{\omega_3}^r C_{\omega_4}^s P_{\mathbf{e}_1, \mathbf{e}_2, \mathbf{e}_3, \mathbf{e}_4}^{p, q, r, s}(0, T, 0) \quad (\text{S37})$$

In our original example for QPT, we considered sixteen possible four-pulse-combination experiments, which can isolate each of the  $P_{\mathbf{e}_1, \mathbf{e}_2, \mathbf{e}_3, \mathbf{e}_4}^{p, q, r, s}(\tau, T, t)$  terms for  $p, q, r, s \in \{\alpha, \beta\}$  for a fixed polarization setting  $(\mathbf{e}_1, \mathbf{e}_2, \mathbf{e}_3, \mathbf{e}_4)$ , which in turn yield enough information to invert the elements of  $\chi(T)$ . The pulses were assumed to be chosen from the toolbox in Eq. 13 in the article. The same sixteen experiments can be extended to the 2D-ES domain by collecting data from many  $\tau$  and  $t$  values, so that  $P_{\mathbf{e}_1, \mathbf{e}_2, \mathbf{e}_3, \mathbf{e}_4}^{p, q, r, s}(0, T, 0) \propto P_{\mathbf{e}_1, \mathbf{e}_2, \mathbf{e}_3, \mathbf{e}_4}^{p, q, r, s}(\tau, T, t)$  can be extracted from Eq. S37, provided that the amplitudes  $S_{ps}(T)$  can be obtained through a fitting procedure of the 2D-ES to a sum of the four lineshapes. However, we can get away with many fewer experiments. The amplitude  $S_{ps}(T)$  only contains information of the Feynman diagrams where the first pulse is centered about  $\omega_{pg}$  and the fourth pulse about  $\omega_{sg}$ . Frequency control over the first and the fourth pulses is redundant, as it will yield 2D-spectra with only one peak at a time. This is unnecessary as each of the four peak amplitudes can be determined independently via a fitting procedure. Instead, a waveform that excites both  $|\alpha\rangle$  and  $|\beta\rangle$  with the same amplitude (e.g., a pulse with carrier frequency in between the excitons,  $\bar{\omega} = \frac{\omega_\alpha + \omega_\beta}{2}$ , and the same  $\sigma$  as before, or shorter) for these two perturbations will, in general, expose the four resonances in a single 2D-ES, so that  $C_{\omega_1}^p = C_{\omega_4}^s$  for all  $p, s$ . However, selective waveforms, such as the ones described for the original QPT, must still be used for the second and third perturbations, as  $S_{ps}(T)$  still contains a sum over  $q, r$ , which needs to be distilled.

The conclusion is that one can trade frequency control for time-delays for the first and fourth pulses, but not for the second and third pulses. For this trade to work, it is essential that no bath-induced coherence transfers occur during the coherence and echo times, so that we can write an optical propagator like Eq. 11 in the article.

## X. SECULAR REDFIELD MODEL FOR MARKOVIAN DISSIPATION

The free evolution of the system  $S$  and bath  $B$  is generated by the total Hamiltonian

$$H_{\text{total}} = H_S + H_B + H_{SB} \quad (\text{S38})$$

where  $H_S$ ,  $H_B$ , and  $H_{SB}$  are the Hamiltonian for  $S$ ,  $B$ , and the interaction between  $S$  and  $B$ , respectively. We model the bath as being constituted by two independent and identically

distributed Ohmic bosonic baths, each linearly coupled to a site of the dimer.

$$\begin{aligned}
H_B &= \sum_{i=\alpha,\beta} \sum_x \omega_{x,i} \left( b_{x,i}^+ b_{x,i} + \frac{1}{2} \right) \\
H_{SB} &= F_\alpha |\alpha\rangle\langle\alpha| + F_\beta |\beta\rangle\langle\beta| + (F_\alpha + F_\beta) |f\rangle\langle f| \\
F_i &= \sum_x \lambda_{x,i} (b_{x,i} + b_{x,i}^+)
\end{aligned} \tag{S39}$$

where  $b_{x,i}$ ,  $b_{x,i}^+$  are the annihilation and creation operators of the bath mode  $x$  coupled to the site  $i$  with frequency  $\omega_{x,i}$ ,  $\lambda_{x,i}$  is a coupling strength, and the spectral density is the same for both sites:

$$\begin{aligned}
J_i(\omega) &= \sum_x \omega_{x,i}^2 \lambda_{x,i}^2 \delta(\omega - \omega_x) \\
&= \frac{\lambda}{\omega_c} \omega e^{-\omega/\omega_c}.
\end{aligned} \tag{S40}$$

We take  $\omega_c = 120 \text{ cm}^{-1}$  and  $\lambda = 30 \text{ cm}^{-1}$ , which are typical energy scales for biomolecular chromophores. By applying second-order perturbation theory on  $H_{SB}$ , tracing over the degrees of freedom of  $B$ , and invoking the Markov and secular approximations, one can arrive at the Redfield equation [17],

$$\dot{\rho}(T) = -i[H_S, \rho(T)] - \mathcal{R}\rho(T), \tag{S41}$$

The Redfield tensor  $\mathcal{R}$  [18] for  $\underline{T} = 273 \text{ K}$  is shown in Table S1. Table S2 shows the explicit expressions of  $\chi(T)$  in terms of  $\mathcal{R}$ .

TABLE S1. Values (in  $\text{ps}^{-1}$ ) of non-zero rates of the (secular) Redfield tensor at  $\underline{T} = 273 \text{ K}$

|                                                                                                       |       |
|-------------------------------------------------------------------------------------------------------|-------|
| $R_{\beta\beta\alpha\alpha}$                                                                          | 2.15  |
| $R_{\alpha\alpha\beta\beta} = e^{-\omega_{\alpha\beta}/k_B \underline{T}} R_{\beta\beta\alpha\alpha}$ | 0.467 |
| $R_{\alpha\beta\alpha\beta} = R_{\beta\alpha\beta\alpha}$                                             | 6.91  |
| $R_{\alpha g \alpha g} = R_{g \alpha g \alpha} = R_{f \alpha f \alpha} = R_{\alpha f \alpha f}$       | 6.95  |
| $R_{\beta g \beta g} = R_{g \beta g \beta} = R_{f \beta f \beta} = R_{\beta f \beta f}$               | 6.11  |
| $R_{f g f g} = R_{g f g f}$                                                                           | 17.9  |

TABLE S2. Analytical expressions for the nonzero elements of  $\chi(T)$  involving single-exciton states

|                                                                           |                                                                |
|---------------------------------------------------------------------------|----------------------------------------------------------------|
| $\chi_{\alpha\alpha\alpha\alpha}(T)$                                      | $e^{-R_{\beta\beta\alpha\alpha}T}$                             |
| $\chi_{\beta\beta\alpha\alpha}(T)$                                        | $1 - e^{-R_{\beta\beta\alpha\alpha}T}$                         |
| $\chi_{\beta\beta\beta\beta}(T)$                                          | $e^{-R_{\alpha\alpha\beta\beta}T}$                             |
| $\chi_{\alpha\alpha\beta\beta}(T)$                                        | $1 - e^{-R_{\alpha\alpha\beta\beta}T}$                         |
| $\chi_{\alpha\beta\alpha\beta}(T) = (\chi_{\beta\alpha\beta\alpha}(T))^*$ | $e^{-i\omega_{\alpha\beta}T} e^{-R_{\alpha\beta\alpha\beta}T}$ |

## XI. RECONSTRUCTION OF $\chi(T)$

We divide the numerical reconstruction of  $\chi(T)$  into two steps.

**A. Reconstruction of the values  $\langle P_{z,z,z,z}^{p,q,r,s}(\tau, T, t) \rangle_{iso}$  from the signals  $\langle [S_{PE}]_{z,z,z,z}^{\omega_1,\omega_2,\omega_3,\omega_4}(\tau, T, t) \rangle_{iso}$**

Eq. (14) in the article can be arranged into a matrix equation,

$$S_{PE}(\tau, T, t) \propto \mathbb{C}P(\tau, T, t) \quad (\text{S42})$$

where  $S_{PE}$  is a vector of the sixteen measured signals  $\langle [S_{PE}]_{z,,e_3,e_4}^{\omega_1,\omega_2,\omega_3,\omega_4}(\tau, T, t) \rangle_{iso}$ ,  $P(\tau, T, t)$  is the vector consisting of the sixteen values  $\langle P_{e_1,e_2,e_3,e_4}^{p,q,r,s}(\tau, T, t) \rangle_{iso}$  which are to be extracted, and  $\mathbb{C}$  is a matrix of known pulse related coefficients  $C_{\omega_1}^p C_{\omega_2}^q C_{\omega_3}^r C_{\omega_4}^s$ . An important issue to address is the stability of the inversion of  $P(\tau, T, t)$  subject to errors in  $S_{PE}(\tau, T, t)$  upon changes in the ratio  $C_2/C_1$  (see Eq. 13 in the article). Denote the spectral norm of a vector or a matrix with  $\| \cdot \|$ . We can bound the errors in the numerically extracted  $P$  from Eq. S42 in terms of the errors in the signal  $S_{PE}$  [19],

$$\frac{\|\Delta P\|}{\|P\|} \leq \kappa_{\mathbb{C}} \frac{\|\Delta S_{PE}\|}{\|S_{PE}\|}, \quad (\text{S43})$$

where  $\Delta P$  and  $\Delta S_{PE}$  are errors in  $P$  and  $S_{PE}$ , respectively. The *condition number*  $\kappa_{\mathbb{C}}$  is given by

$$\kappa_{\mathbb{C}} = \| \mathbb{C}(T) \| \| [\mathbb{C}(T)]^{-1} \|, \quad (\text{S44})$$

yields a measure of the amplification of the relative errors on the inverted vector due to the relative errors in the experimental data. The lowest possible value for a condition number is 1. When both waveforms of the toolbox excite  $|\alpha\rangle$  and  $|\beta\rangle$  with the same amplitude ( $C'/C'' = 1$ ), there is no selectivity in the preparation and detection of states in the energy domain, and  $\kappa_{\mathbb{C}} = \infty$ , yielding the worst scenario for reconstruction. The best scenario occurs for the MDC case ( $C'/C'' \rightarrow \infty$ ), where  $\mathbb{C}$  is proportional to the identity matrix, and  $\kappa_{\mathbb{C}} = 1$ .

Not surprisingly,  $\kappa_{\mathbb{C}}$  decreases monotonically over the  $C'/C'' \in [1, \infty]$  range. Fig. S1 shows  $\kappa_{\mathbb{C}}$  with respect to  $C'/C''$ . The small values of  $\kappa_{\mathbb{C}}$  imply a robust numerical extraction of  $P(\tau, T, t)$  over a wide range of obtainable  $C'/C''$ .

**B. Reconstruction of  $\chi(T)$  from  $\langle P_{z,z,z,z}^{p,q,r,s}(\tau, T, t) \rangle_{iso}$**

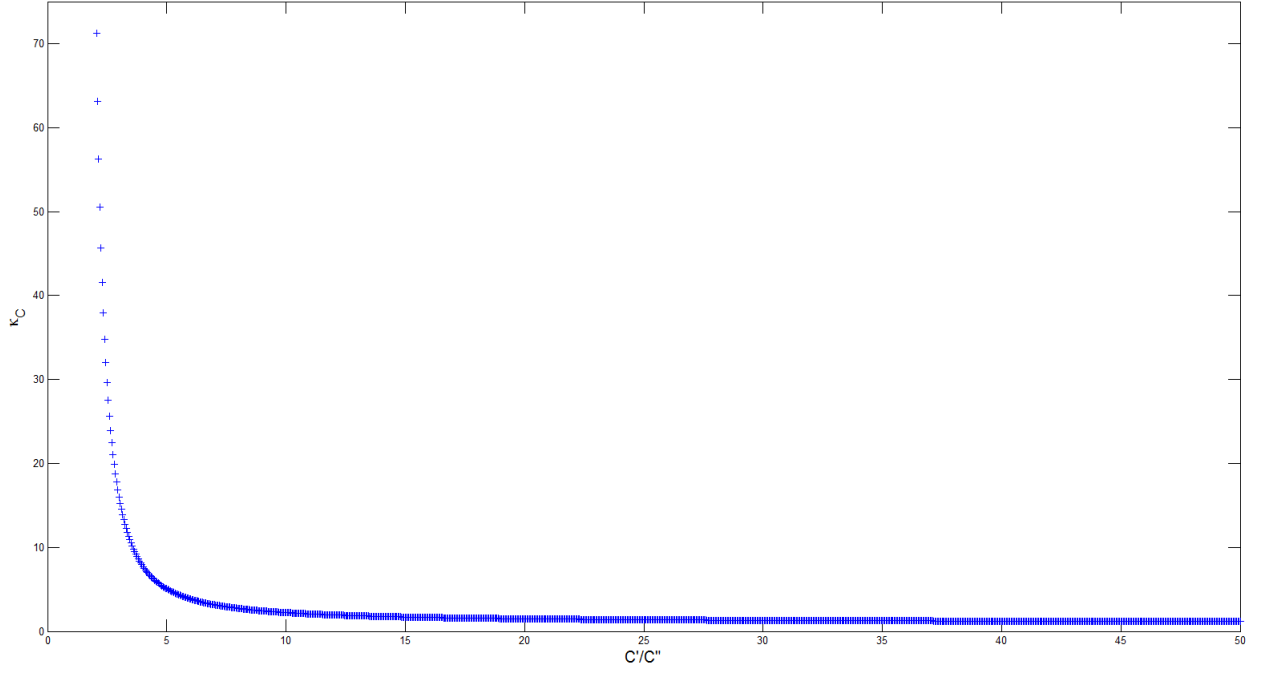

Figure S2: *Plot of  $\kappa_C$  vs.  $C'/C''$ .* The function decreases monotonically over  $C'/C'' \in [1, \infty]$ , as expected, with  $C'/C'' = 1$  being the worst scenario of reconstruction corresponding to the case of equal pulse amplitude at both excitonic energies  $\omega_{\alpha g}$  and  $\omega_{\beta g}$ , and  $C'/C'' = \infty$  being the best scenario corresponding to the MDC.

Table S3. A set of experiments which yields  $\chi(T)$ 

| From the data                                                                                                                                                                                                                                                                                                                                                                                                                                                                                                                                                                                                                                                                               | we can reconstruct the elements                             | which explicitly listed are                                                                                                                                                                                                                                                                                                                                                                                                                                                                                                                                                                                                                                                                                                                                     |
|---------------------------------------------------------------------------------------------------------------------------------------------------------------------------------------------------------------------------------------------------------------------------------------------------------------------------------------------------------------------------------------------------------------------------------------------------------------------------------------------------------------------------------------------------------------------------------------------------------------------------------------------------------------------------------------------|-------------------------------------------------------------|-----------------------------------------------------------------------------------------------------------------------------------------------------------------------------------------------------------------------------------------------------------------------------------------------------------------------------------------------------------------------------------------------------------------------------------------------------------------------------------------------------------------------------------------------------------------------------------------------------------------------------------------------------------------------------------------------------------------------------------------------------------------|
| $\left\{ \begin{array}{l} \langle P_{z,z,z,z}^{\alpha,\alpha,\alpha}(\tau, T, t) \rangle_{iso}, \\ \langle P_{z,z,z,z}^{\alpha,\alpha,\beta}(\tau, T, t) \rangle_{iso}, \\ \langle P_{z,z,z,z}^{\alpha,\beta,\beta}(\tau, T, t) \rangle_{iso}, \\ \langle P_{z,z,z,z}^{\alpha,\beta,\alpha}(\tau, T, t) \rangle_{iso} \end{array} \right\}$                                                                                                                                                                                                                                                                                                                                                 | $\{\chi_{ij\alpha\alpha}(T)\}$                              | $\left\{ \begin{array}{l} \chi_{\alpha\alpha\alpha\alpha}(T), \\ \chi_{\beta\beta\alpha\alpha}(T), \\ \Re\{\chi_{\alpha\beta\alpha\alpha}(T)\} = \Re\{\chi_{\beta\alpha\alpha\alpha}(T)\}, \\ \Im\{\chi_{\alpha\beta\alpha\alpha}(T)\} = -\Im\{\chi_{\beta\alpha\alpha\alpha}(T)\} \end{array} \right\}$                                                                                                                                                                                                                                                                                                                                                                                                                                                        |
| $\left\{ \begin{array}{l} \langle P_{z,z,z,z}^{\beta,\beta,\alpha,\alpha}(\tau, T, t) \rangle_{iso}, \\ \langle P_{z,z,z,z}^{\beta,\beta,\alpha,\beta}(\tau, T, t) \rangle_{iso}, \\ \langle P_{z,z,z,z}^{\beta,\beta,\beta,\beta}(\tau, T, t) \rangle_{iso}, \\ \langle P_{z,z,z,z}^{\beta,\beta,\alpha,\beta}(\tau, T, t) \rangle_{iso} \end{array} \right\}$                                                                                                                                                                                                                                                                                                                             | $\{\chi_{ij\beta\beta}(T)\}$                                | $\left\{ \begin{array}{l} \chi_{\alpha\alpha\beta\beta}(T), \\ \chi_{\beta\beta\beta\beta}(T), \\ \Re\{\chi_{\alpha\beta\beta\beta}(T)\} = \Re\{\chi_{\beta\alpha\beta\beta}(T)\}, \\ \Im\{\chi_{\alpha\beta\beta\beta}(T)\} = -\Im\{\chi_{\beta\alpha\beta\beta}(T)\} \end{array} \right\}$                                                                                                                                                                                                                                                                                                                                                                                                                                                                    |
| $\left\{ \begin{array}{l} \langle P_{z,z,z,z}^{\beta,\alpha,\alpha,\alpha}(\tau, T, t) \rangle_{iso}, \\ \langle P_{z,z,z,z}^{\beta,\alpha,\alpha,\beta}(\tau, T, t) \rangle_{iso}, \\ \langle P_{z,x,x,z}^{\beta,\alpha,\beta,\beta}(\tau, T, t) \rangle_{iso}, \\ \langle P_{z,x,x,z}^{\beta,\alpha,\beta,\alpha}(\tau, T, t) \rangle_{iso}, \\ \langle P_{z,z,z,z}^{\alpha,\beta,\alpha,\alpha}(\tau, T, t) \rangle_{iso}, \\ \langle P_{z,z,z,z}^{\alpha,\beta,\alpha,\beta}(\tau, T, t) \rangle_{iso}, \\ \langle P_{z,z,z,z}^{\alpha,\beta,\beta,\beta}(\tau, T, t) \rangle_{iso}, \\ \langle P_{z,z,z,z}^{\alpha,\beta,\beta,\alpha}(\tau, T, t) \rangle_{iso} \end{array} \right\}$ | $\{\chi_{ij\alpha\beta}(T) = (\chi_{ji\beta\alpha}(T))^*\}$ | $\left\{ \begin{array}{l} \Re\{\chi_{\alpha\alpha\alpha\beta}(T)\} = \Re\{\chi_{\alpha\alpha\beta\alpha}(T)\}, \\ \Im\{\chi_{\alpha\alpha\alpha\beta}(T)\} = -\Im\{\chi_{\alpha\alpha\beta\alpha}(T)\}, \\ \Re\{\chi_{\beta\beta\alpha\beta}(T)\} = \Re\{\chi_{\beta\beta\beta\alpha}(T)\}, \\ \Im\{\chi_{\beta\beta\alpha\beta}(T)\} = -\Im\{\chi_{\beta\beta\beta\alpha}(T)\}, \\ \Re\{\chi_{\alpha\beta\alpha\beta}(T)\} = \Re\{\chi_{\beta\alpha\beta\alpha}(T)\}, \\ \Im\{\chi_{\alpha\beta\alpha\beta}(T)\} = -\Im\{\chi_{\beta\alpha\beta\alpha}(T)\}, \\ \Re\{\chi_{\beta\alpha\alpha\beta}(T)\} = \Re\{\chi_{\alpha\beta\alpha\beta}(T)\}, \\ \Im\{\chi_{\beta\alpha\alpha\beta}(T)\} = -\Im\{\chi_{\alpha\beta\alpha\beta}(T)\} \end{array} \right\}$ |

Once the  $\langle P_{z,z,z,z}^{p,q,r,s}(\tau, T, t) \rangle_{iso}$  values have been extracted, a second step to extract  $\chi(T)$  from them is required. The explicit trace preservation identities,

$$\begin{aligned}
 \chi_{gg\alpha\alpha}(T) - 1 &= -\chi_{\alpha\alpha\alpha\alpha}(T) - \chi_{\beta\beta\alpha\alpha}(T), \\
 \chi_{gg\beta\beta}(T) - 1 &= -\chi_{\alpha\alpha\beta\beta}(T) - \chi_{\beta\beta\beta\beta}(T), \\
 \Re\{\chi_{gg\alpha\beta}(T)\} &= -\Re\{\chi_{\alpha\alpha\alpha\beta}(T)\} - \Re\{\chi_{\beta\beta\alpha\beta}(T)\}, \\
 \Im\{\chi_{gg\alpha\beta}(T)\} &= -\Im\{\chi_{\alpha\alpha\alpha\beta}(T)\} - \Im\{\chi_{\beta\beta\alpha\beta}(T)\},
 \end{aligned} \tag{S45}$$

together with the Hermiticity identities in column 2 of Table S3, can be substituted into Eqs. 14-16 in the article, and their analogues upon the  $\alpha \leftrightarrow \beta$  substitution. After isotropic averaging, we can write the matrix equations,

$$\mathbb{M}^{qp} X^{qp}(T) = P^{qp}(T), \tag{S46}$$

each of them corresponding to an initial state  $qp$ . The analytical expressions of the square matrices  $\mathbb{M}^{qp}$  are listed in Tables S4, S5, and S6. The real vectors  $X$  to extract contain the

elements of the process matrix,

$$\begin{aligned}
X^{\alpha\alpha}(T) &= \begin{bmatrix} \chi_{\alpha\alpha\alpha\alpha}(T) \\ \chi_{\beta\beta\alpha\alpha}(T) \\ \Re\{\chi_{\alpha\beta\alpha\alpha}(T)\} \\ \Im\{\chi_{\alpha\beta\alpha\alpha}(T)\} \end{bmatrix}, \\
X^{\beta\beta}(T) &= \begin{bmatrix} \chi_{\alpha\alpha\beta\beta}(T) \\ \chi_{\beta\beta\beta\beta}(T) \\ \Re\{\chi_{\alpha\beta\beta\beta}(T)\} \\ \Im\{\chi_{\alpha\beta\beta\beta}(T)\} \end{bmatrix}, \\
X^{\alpha\beta}(T) &= \begin{bmatrix} \Re\{\chi_{\alpha\alpha\alpha\beta}(T)\} \\ \Re\{\chi_{\beta\beta\alpha\beta}(T)\} \\ \Re\{\chi_{\alpha\beta\alpha\beta}(T)\} \\ \Re\{\chi_{\beta\alpha\alpha\beta}(T)\} \\ \Im\{\chi_{\alpha\alpha\alpha\beta}(T)\} \\ \Im\{\chi_{\beta\beta\alpha\beta}(T)\} \\ \Im\{\chi_{\alpha\beta\alpha\beta}(T)\} \\ \Im\{\chi_{\beta\alpha\alpha\beta}(T)\} \end{bmatrix}, \tag{S47}
\end{aligned}$$

whereas the vectors consisting of data from experiments are

$$\begin{aligned}
P^{\alpha\alpha}(T) &= \begin{bmatrix} \langle P^{\alpha,\alpha,\alpha,\alpha}(0, T, 0) \rangle_{iso} \\ \langle P^{\alpha,\alpha,\alpha,\beta}(0, T, 0) \rangle_{iso} \\ \langle P^{\alpha,\alpha,\beta,\alpha}(0, T, 0) \rangle_{iso} \\ \langle P^{\alpha,\alpha,\beta,\beta}(0, T, 0) \rangle_{iso} \end{bmatrix}, \\
P^{\beta\beta}(T) &= \begin{bmatrix} \langle P^{\beta,\beta,\alpha,\alpha}(0, T, 0) \rangle_{iso} \\ \langle P^{\beta,\beta,\alpha,\beta}(0, T, 0) \rangle_{iso} \\ \langle P^{\beta,\beta,\beta,\alpha}(0, T, 0) \rangle_{iso} \\ \langle P^{\beta,\beta,\beta,\beta}(0, T, 0) \rangle_{iso} \end{bmatrix}, \\
P^{\alpha\beta}(T) &= \begin{bmatrix} \langle P^{\beta,\alpha,\alpha,\alpha}(0, T, 0) \rangle_{iso} \\ \langle P^{\beta,\alpha,\alpha,\beta}(0, T, 0) \rangle_{iso} \\ \langle P^{\beta,\alpha,\beta,\alpha}(0, T, 0) \rangle_{iso} \\ \langle P^{\beta,\alpha,\beta,\beta}(0, T, 0) \rangle_{iso} \\ \langle P^{\alpha,\beta,\alpha,\alpha}(0, T, 0) \rangle_{iso} \\ \langle P^{\alpha,\beta,\alpha,\beta}(0, T, 0) \rangle_{iso} \\ \langle P^{\alpha,\beta,\beta,\alpha}(0, T, 0) \rangle_{iso} \\ \langle P^{\alpha,\beta,\beta,\beta}(0, T, 0) \rangle_{iso} \end{bmatrix}.
\end{aligned}$$

Construction of the  $P^{qp}(T)$  vectors can be done from the values  $\langle P_{z,z,z,z}^{p,q,r,s}(0, T, 0) \rangle_{iso}$  stemming from TD/TB measurements, or alternatively, after factoring the coherence and echo propagators from the values  $\langle P_{z,z,z,z}^{p,q,r,s}(\tau, T, t) \rangle_{iso}$  given by the general rephasing PE experiment, as in Eq. S32.

| Table S4. Entries of $\mathbb{M}^{\alpha\alpha}$ |        |                                                                                                                                                                                                                         |
|--------------------------------------------------|--------|-------------------------------------------------------------------------------------------------------------------------------------------------------------------------------------------------------------------------|
| ROW                                              | COLUMN | VALUE                                                                                                                                                                                                                   |
| 1                                                | 1      | $\frac{2\mu_{\alpha g}^4}{5}$                                                                                                                                                                                           |
| 1                                                | 2      | $\frac{\mu_{\alpha g}^4}{5} - \frac{1}{15} (\cos(2\theta_{f\beta}) + 2) \mu_{f\beta}^2 \mu_{\alpha g}^2$                                                                                                                |
| 1                                                | 3      | 0                                                                                                                                                                                                                       |
| 1                                                | 4      | 0                                                                                                                                                                                                                       |
| 2                                                | 1      | 0                                                                                                                                                                                                                       |
| 2                                                | 2      | 0                                                                                                                                                                                                                       |
| 2                                                | 3      | $\frac{1}{15} \mu_{\alpha g}^2 (3 \cos(\theta_{\beta g}) \mu_{\alpha g} \mu_{\beta g} - (3 \cos(\theta_{f\alpha}) \cos(\theta_{f\beta}) + \sin(\theta_{f\alpha}) \sin(\theta_{f\beta})) \mu_{f\alpha} \mu_{f\beta})$    |
| 2                                                | 4      | $\frac{1}{15} i \mu_{\alpha g}^2 ((3 \cos(\theta_{f\alpha}) \cos(\theta_{f\beta}) + \sin(\theta_{f\alpha}) \sin(\theta_{f\beta})) \mu_{f\alpha} \mu_{f\beta} - 3 \cos(\theta_{\beta g}) \mu_{\alpha g} \mu_{\beta g})$  |
| 3                                                | 1      | 0                                                                                                                                                                                                                       |
| 3                                                | 2      | 0                                                                                                                                                                                                                       |
| 3                                                | 3      | $\frac{1}{15} \mu_{\alpha g}^2 (3 \cos(\theta_{\beta g}) \mu_{\alpha g} \mu_{\beta g} - (3 \cos(\theta_{f\alpha}) \cos(\theta_{f\beta}) + \sin(\theta_{f\alpha}) \sin(\theta_{f\beta})) \mu_{f\alpha} \mu_{f\beta})$    |
| 3                                                | 4      | $-\frac{1}{15} i \mu_{\alpha g}^2 ((3 \cos(\theta_{f\alpha}) \cos(\theta_{f\beta}) + \sin(\theta_{f\alpha}) \sin(\theta_{f\beta})) \mu_{f\alpha} \mu_{f\beta} - 3 \cos(\theta_{\beta g}) \mu_{\alpha g} \mu_{\beta g})$ |
| 4                                                | 1      | $\frac{1}{15} \mu_{\alpha g}^2 ((\cos(2\theta_{\beta g}) + 2) \mu_{\beta g}^2 - (\cos(2\theta_{f\alpha}) + 2) \mu_{f\alpha}^2)$                                                                                         |
| 4                                                | 2      | $\frac{2}{15} (\cos(2\theta_{\beta g}) + 2) \mu_{\alpha g}^2 \mu_{\beta g}^2$                                                                                                                                           |
| 4                                                | 3      | 0                                                                                                                                                                                                                       |
| 4                                                | 4      | 0                                                                                                                                                                                                                       |

| Table S5. Entries of $\mathbb{M}^{\beta\beta}$ |        |                                                                                                                                                                                                                                   |
|------------------------------------------------|--------|-----------------------------------------------------------------------------------------------------------------------------------------------------------------------------------------------------------------------------------|
| ROW                                            | COLUMN | VALUE                                                                                                                                                                                                                             |
| 1                                              | 1      | $\frac{2}{15} (\cos(2\theta_{\beta g}) + 2) \mu_{\alpha g}^2 \mu_{\beta g}^2$                                                                                                                                                     |
| 1                                              | 2      | $\frac{1}{15} ((\cos(2\theta_{\beta g}) + 2) \mu_{\alpha g}^2 - (\cos(2(\theta_{f\beta} - \theta_{\beta g})) + 2) \mu_{f\beta}^2) \mu_{\beta g}^2$                                                                                |
| 1                                              | 3      | 0                                                                                                                                                                                                                                 |
| 1                                              | 4      | 0                                                                                                                                                                                                                                 |
| 2                                              | 1      | 0                                                                                                                                                                                                                                 |
| 2                                              | 2      | 0                                                                                                                                                                                                                                 |
| 2                                              | 3      | $\frac{1}{15} \mu_{\beta g}^2 (3 \cos(\theta_{\beta g}) \mu_{\alpha g} \mu_{\beta g} - (2 \cos(\theta_{f\alpha} - \theta_{f\beta}) + \cos(\theta_{f\alpha} + \theta_{f\beta} - 2\theta_{\beta g})) \mu_{f\alpha} \mu_{f\beta})$   |
| 2                                              | 4      | $\frac{1}{15} i \mu_{\beta g}^2 ((2 \cos(\theta_{f\alpha} - \theta_{f\beta}) + \cos(\theta_{f\alpha} + \theta_{f\beta} - 2\theta_{\beta g})) \mu_{f\alpha} \mu_{f\beta} - 3 \cos(\theta_{\beta g}) \mu_{\alpha g} \mu_{\beta g})$ |
| 3                                              | 1      | 0                                                                                                                                                                                                                                 |
| 3                                              | 2      | 0                                                                                                                                                                                                                                 |
| 3                                              | 3      | $\frac{1}{15} \mu_{\beta g}^2 (3 \cos(\theta_{\beta g}) \mu_{\alpha g} \mu_{\beta g} - (2 \cos(\theta_{f\alpha} - \theta_{f\beta}) + \cos(\theta_{f\alpha} + \theta_{f\beta} - 2\theta_{\beta g})) \mu_{f\alpha} \mu_{f\beta})$   |
| 3                                              | 4      | $\frac{1}{15} i \mu_{\beta g}^2 (3 \cos(\theta_{\beta g}) \mu_{\alpha g} \mu_{\beta g} - (2 \cos(\theta_{f\alpha} - \theta_{f\beta}) + \cos(\theta_{f\alpha} + \theta_{f\beta} - 2\theta_{\beta g})) \mu_{f\alpha} \mu_{f\beta})$ |
| 4                                              | 1      | $\frac{1}{15} \mu_{\beta g}^2 (3 \mu_{\beta g}^2 - (\cos(2(\theta_{f\alpha} - \theta_{\beta g})) + 2) \mu_{f\alpha}^2)$                                                                                                           |
| 4                                              | 2      | $\frac{2\mu_{\beta g}^4}{5}$                                                                                                                                                                                                      |
| 4                                              | 3      | 0                                                                                                                                                                                                                                 |
| 4                                              | 4      | 0                                                                                                                                                                                                                                 |



Table S6. Entries of  $\mathbb{M}^{\alpha\beta}$ 

| ROW | COLUMN | VALUE                                                                                                                                                                                                                                                                     |
|-----|--------|---------------------------------------------------------------------------------------------------------------------------------------------------------------------------------------------------------------------------------------------------------------------------|
| 1   | 1      | $\frac{2}{5} \cos(\theta_{\beta g}) \mu_{\alpha g}^3 \mu_{\beta g}$                                                                                                                                                                                                       |
| 1   | 2      | $\frac{1}{15} \mu_{\alpha g} \left( 3 \cos(\theta_{\beta g}) \mu_{\alpha g}^2 - (\cos(2\theta_{f\beta} - \theta_{\beta g}) + 2 \cos(\theta_{\beta g})) \mu_{f\beta}^2 \right) \mu_{\beta g}$                                                                              |
| 1   | 3      | 0                                                                                                                                                                                                                                                                         |
| 1   | 4      | 0                                                                                                                                                                                                                                                                         |
| 1   | 5      | $\frac{2}{5} i \cos(\theta_{\beta g}) \mu_{\alpha g}^3 \mu_{\beta g}$                                                                                                                                                                                                     |
| 1   | 6      | $-\frac{1}{15} i \mu_{\alpha g} \left( (\cos(2\theta_{f\beta} - \theta_{\beta g}) + 2 \cos(\theta_{\beta g})) \mu_{f\beta}^2 - 3 \cos(\theta_{\beta g}) \mu_{\alpha g}^2 \right) \mu_{\beta g}$                                                                           |
| 1   | 7      | 0                                                                                                                                                                                                                                                                         |
| 1   | 8      | 0                                                                                                                                                                                                                                                                         |
| 2   | 1      | 0                                                                                                                                                                                                                                                                         |
| 2   | 2      | 0                                                                                                                                                                                                                                                                         |
| 2   | 3      | 0                                                                                                                                                                                                                                                                         |
| 2   | 4      | $\frac{1}{15} \mu_{\alpha g} \mu_{\beta g} ((\cos(2\theta_{\beta g}) + 2) \mu_{\alpha g} \mu_{\beta g} - (\cos(\theta_{f\alpha} - \theta_{f\beta} - \theta_{\beta g}) + 2 \cos(\theta_{f\alpha}) \cos(\theta_{f\beta} - \theta_{\beta g})) \mu_{f\alpha} \mu_{f\beta})$   |
| 2   | 5      | 0                                                                                                                                                                                                                                                                         |
| 2   | 6      | 0                                                                                                                                                                                                                                                                         |
| 2   | 7      | 0                                                                                                                                                                                                                                                                         |
| 2   | 8      | $\frac{1}{15} i \mu_{\alpha g} \mu_{\beta g} ((\cos(2\theta_{\beta g}) + 2) \mu_{\alpha g} \mu_{\beta g} - (\cos(\theta_{f\alpha} - \theta_{f\beta} - \theta_{\beta g}) + 2 \cos(\theta_{f\alpha}) \cos(\theta_{f\beta} - \theta_{\beta g})) \mu_{f\alpha} \mu_{f\beta})$ |
| 3   | 1      | 0                                                                                                                                                                                                                                                                         |
| 3   | 2      | 0                                                                                                                                                                                                                                                                         |
| 3   | 3      | $\frac{1}{15} \mu_{\alpha g} \mu_{\beta g} ((\cos(2\theta_{\beta g}) + 2) \mu_{\alpha g} \mu_{\beta g} - (\cos(\theta_{f\alpha} - \theta_{f\beta} - \theta_{\beta g}) + 2 \cos(\theta_{f\alpha}) \cos(\theta_{f\beta} - \theta_{\beta g})) \mu_{f\alpha} \mu_{f\beta})$   |
| 3   | 4      | 0                                                                                                                                                                                                                                                                         |
| 3   | 5      | 0                                                                                                                                                                                                                                                                         |
| 3   | 6      | 0                                                                                                                                                                                                                                                                         |
| 3   | 7      | $\frac{1}{15} i \mu_{\alpha g} \mu_{\beta g} ((\cos(2\theta_{\beta g}) + 2) \mu_{\alpha g} \mu_{\beta g} - (\cos(\theta_{f\alpha} - \theta_{f\beta} - \theta_{\beta g}) + 2 \cos(\theta_{f\alpha}) \cos(\theta_{f\beta} - \theta_{\beta g})) \mu_{f\alpha} \mu_{f\beta})$ |
| 3   | 8      | 0                                                                                                                                                                                                                                                                         |
| 4   | 1      | $\frac{1}{15} \mu_{\alpha g} \mu_{\beta g} \left( 3 \cos(\theta_{\beta g}) \mu_{\beta g}^2 - (\cos(2\theta_{f\alpha} - \theta_{\beta g}) + 2 \cos(\theta_{\beta g})) \mu_{f\alpha}^2 \right)$                                                                             |
| 4   | 2      | $\frac{2}{5} \cos(\theta_{\beta g}) \mu_{\alpha g} \mu_{\beta g}^3$                                                                                                                                                                                                       |
| 4   | 3      | 0                                                                                                                                                                                                                                                                         |
| 4   | 4      | 0                                                                                                                                                                                                                                                                         |
| 4   | 5      | $-\frac{1}{15} i \mu_{\alpha g} \mu_{\beta g} \left( (\cos(2\theta_{f\alpha} - \theta_{\beta g}) + 2 \cos(\theta_{\beta g})) \mu_{f\alpha}^2 - 3 \cos(\theta_{\beta g}) \mu_{\beta g}^2 \right)$                                                                          |
| 4   | 6      | $\frac{2}{5} i \cos(\theta_{\beta g}) \mu_{\alpha g} \mu_{\beta g}^3$                                                                                                                                                                                                     |
| 4   | 7      | 0                                                                                                                                                                                                                                                                         |
| 4   | 8      | 0                                                                                                                                                                                                                                                                         |

| Table S6 (continued). Entries of $\mathbb{M}^{\alpha\beta}$ |        |                                                                                                                                                                                                                                                |
|-------------------------------------------------------------|--------|------------------------------------------------------------------------------------------------------------------------------------------------------------------------------------------------------------------------------------------------|
| ROW                                                         | COLUMN | VALUE                                                                                                                                                                                                                                          |
| 5                                                           | 1      | $\frac{2}{5} \cos(\theta_{\beta g}) \mu_{\alpha g}^3 \mu_{\beta g}$                                                                                                                                                                            |
| 5                                                           | 2      | $\frac{1}{15} \mu_{\alpha g} \left( 3 \cos(\theta_{\beta g}) \mu_{\alpha g}^2 - (\cos(2\theta_{fg} - \theta_{\beta g}) + 2 \cos(\theta_{\beta g})) \mu_{fg}^2 \right) \mu_{\beta g}$                                                           |
| 5                                                           | 3      | 0                                                                                                                                                                                                                                              |
| 5                                                           | 4      | 0                                                                                                                                                                                                                                              |
| 5                                                           | 5      | $-\frac{2}{5} i \cos(\theta_{\beta g}) \mu_{\alpha g}^3 \mu_{\beta g}$                                                                                                                                                                         |
| 5                                                           | 6      | $\frac{1}{15} i \mu_{\alpha g} \left( (\cos(2\theta_{fg} - \theta_{\beta g}) + 2 \cos(\theta_{\beta g})) \mu_{fg}^2 - 3 \cos(\theta_{\beta g}) \mu_{\alpha g}^2 \right) \mu_{\beta g}$                                                         |
| 5                                                           | 7      | 0                                                                                                                                                                                                                                              |
| 5                                                           | 8      | 0                                                                                                                                                                                                                                              |
| 6                                                           | 1      | 0                                                                                                                                                                                                                                              |
| 6                                                           | 2      | 0                                                                                                                                                                                                                                              |
| 6                                                           | 3      | $\frac{1}{15} \mu_{\alpha g} \mu_{\beta g} ((\cos(2\theta_{\beta g}) + 2) \mu_{\alpha g} \mu_{\beta g} - (\cos(\theta_{fg} - \theta_{fg} - \theta_{\beta g}) + 2 \cos(\theta_{fg}) \cos(\theta_{fg} - \theta_{\beta g})) \mu_{fg} \mu_{fg})$   |
| 6                                                           | 4      | 0                                                                                                                                                                                                                                              |
| 6                                                           | 5      | 0                                                                                                                                                                                                                                              |
| 6                                                           | 6      | 0                                                                                                                                                                                                                                              |
| 6                                                           | 7      | $\frac{1}{15} i \mu_{\alpha g} \mu_{\beta g} ((\cos(\theta_{fg} - \theta_{fg} - \theta_{\beta g}) + 2 \cos(\theta_{fg}) \cos(\theta_{fg} - \theta_{\beta g})) \mu_{fg} \mu_{fg} - (\cos(2\theta_{\beta g}) + 2) \mu_{\alpha g} \mu_{\beta g})$ |
| 6                                                           | 8      | 0                                                                                                                                                                                                                                              |
| 7                                                           | 1      | 0                                                                                                                                                                                                                                              |
| 7                                                           | 2      | 0                                                                                                                                                                                                                                              |
| 7                                                           | 3      | 0                                                                                                                                                                                                                                              |
| 7                                                           | 4      | $\frac{1}{15} \mu_{\alpha g} \mu_{\beta g} ((\cos(2\theta_{\beta g}) + 2) \mu_{\alpha g} \mu_{\beta g} - (\cos(\theta_{fg} - \theta_{fg} - \theta_{\beta g}) + 2 \cos(\theta_{fg}) \cos(\theta_{fg} - \theta_{\beta g})) \mu_{fg} \mu_{fg})$   |
| 7                                                           | 5      | 0                                                                                                                                                                                                                                              |
| 7                                                           | 6      | 0                                                                                                                                                                                                                                              |
| 7                                                           | 7      | 0                                                                                                                                                                                                                                              |
| 7                                                           | 8      | $\frac{1}{15} i \mu_{\alpha g} \mu_{\beta g} ((\cos(\theta_{fg} - \theta_{fg} - \theta_{\beta g}) + 2 \cos(\theta_{fg}) \cos(\theta_{fg} - \theta_{\beta g})) \mu_{fg} \mu_{fg} - (\cos(2\theta_{\beta g}) + 2) \mu_{\alpha g} \mu_{\beta g})$ |
| 8                                                           | 1      | $\frac{1}{15} \mu_{\alpha g} \mu_{\beta g} (3 \cos(\theta_{\beta g}) \mu_{\beta g}^2 - (\cos(2\theta_{fg} - \theta_{\beta g}) + 2 \cos(\theta_{\beta g})) \mu_{fg}^2)$                                                                         |
| 8                                                           | 2      | $\frac{2}{5} \cos(\theta_{\beta g}) \mu_{\alpha g} \mu_{\beta g}^3$                                                                                                                                                                            |
| 8                                                           | 3      | 0                                                                                                                                                                                                                                              |
| 8                                                           | 4      | 0                                                                                                                                                                                                                                              |
| 8                                                           | 5      | $\frac{1}{15} i \mu_{\alpha g} \mu_{\beta g} ((\cos(2\theta_{fg} - \theta_{\beta g}) + 2 \cos(\theta_{\beta g})) \mu_{fg}^2 - 3 \cos(\theta_{\beta g}) \mu_{\beta g}^2)$                                                                       |
| 8                                                           | 6      | $-\frac{2}{5} i \cos(\theta_{\beta g}) \mu_{\alpha g} \mu_{\beta g}^3$                                                                                                                                                                         |
| 8                                                           | 7      | 0                                                                                                                                                                                                                                              |
| 8                                                           | 8      | 0                                                                                                                                                                                                                                              |

The matrices  $\mathbb{M}^{qp}$  can be easily reexpressed in terms of  $d_A$ ,  $d_B$ ,  $\phi$ , and  $\theta$  using the equations in section I. As in subsection A, we obtain a bound on the relative error of  $X^{qp}(T)$  [19, 20]:

$$\frac{\|\Delta X^{qp}(T)\|}{\|X^{qp}(T)\|} \leq \kappa^{qp} \frac{\|\Delta P^{qp}(T)\|}{\|P^{qp}(T)\|}. \quad (\text{S48})$$

The condition number  $\kappa^{qp}$  is given by,

$$\kappa^{qp} = \|\mathbb{M}^{qp}\| \|\mathbb{M}^{qp}\|^{-1}. \quad (\text{S49})$$

Fig. S2 shows contour plots of  $\kappa \equiv \max_{qp} \kappa$  for a set of fixed dipole norm ratios  $d_B/d_A$  across the entire range of angles  $0 \leq \theta, \phi < \pi$ . For  $d_B/d_A = 1$  (panel (a)), there are four stripes for which the QPT protocol fails. The stripes along  $\theta = 0, \frac{\pi}{2}$  correspond to the absence of excitonic coupling ( $J = 0$ ), whereas the ones along  $\theta = \frac{\pi}{4}, \frac{3\pi}{4}$  correspond to the homodimer

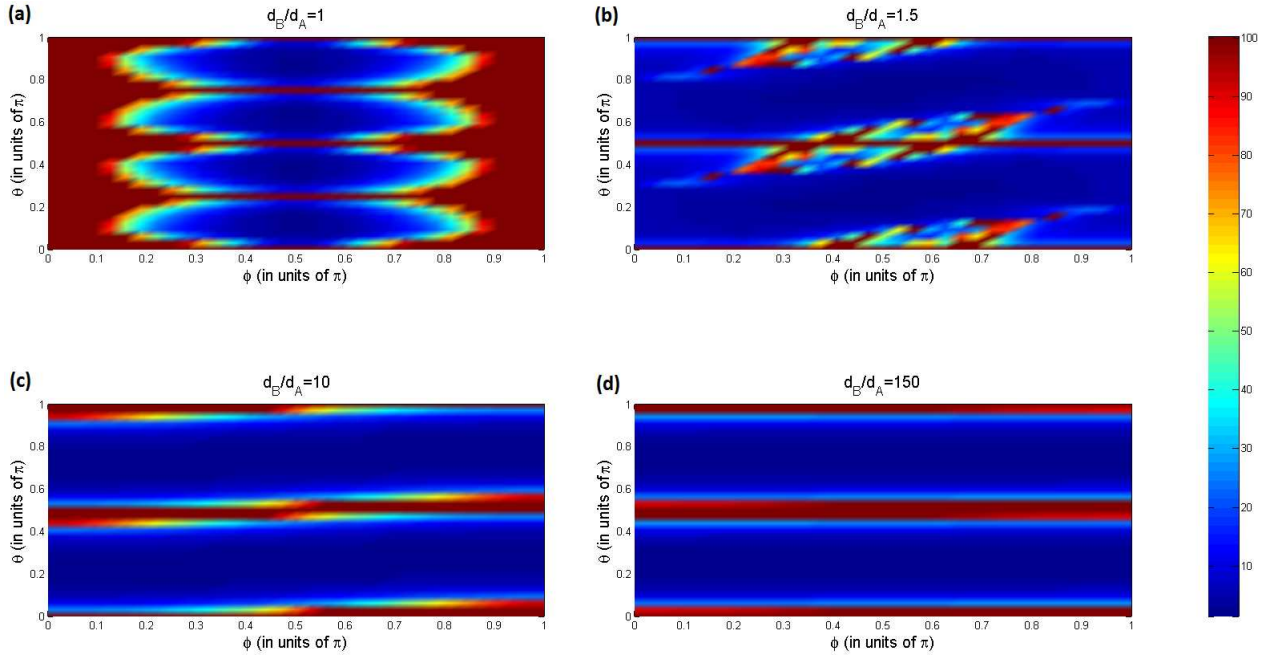

Figure S3: *Contour plots of  $\kappa$  vs.  $\theta$  and  $\phi$ .* The stripes about  $\theta = 0, \frac{\pi}{2}$  correspond to the case of uncoupled chromophores, and fail to provide a QPT via our suggested protocol. Additional unstable regions emerge about  $\theta = \frac{\pi}{4}, \frac{3\pi}{4}$  for  $d_B/d_A = 1$  (panel (a)), which correspond to the homodimer case. The  $\theta = \pi$  case is equivalent to the  $\theta = 0$  case. Note that beyond the unstable regions, QPT is very robust, with condition number  $\kappa$  values on the order of 1 to 10.

case. As explained in Ref. [4], isotropic averages of signal denoting coherence to population or opposite processes vanish for a homodimer. Therefore, QPT is incomplete in those cases and large condition numbers arise near those critical angles. QPT is, however, quite robust in the wide range of structural parameters which do not lie in the critical stripes, with  $\kappa$  values on the order of 1 to 10. For  $d_B/d_A = 1.5, 10, 100$  (panels (b), (c) and (d)), there is no possibility of homodimer, and in fact, the inversion only fails for the uncoupled chromophores situation. In general, the  $\kappa$  dependence on  $\theta, \phi$  is seen to be largely insensitive to the ratio  $d_B/d_A \neq 1$ . This phenomenon can be easily understood as follows: as long as there is coupling between the site excitons, the oscillator strength is fairly distributed between the two eigenstates of the single-exciton manifold even if their site oscillator strengths differ by many orders of magnitude.

Remarkably, the protocol does not fail for the  $\phi = 0, \pi$  cases, when the site dipoles are aligned or antialigned, except when  $d_B/d_A = 1$ . For the latter, it happens that  $\boldsymbol{\mu}_{\alpha g} = \boldsymbol{\mu}_{f\alpha}$  and  $\boldsymbol{\mu}_{\beta g} = \boldsymbol{\mu}_{f\beta}$ , yielding singular matrices  $\mathbb{M}^{qp}$ . For these particular  $\phi$  values and general  $d_B/d_A$  ratios, the four parallel transition dipoles have different magnitude but the same direction. Since the currently proposed spectroscopic addressing of the states is through frequency space rather than through polarization, these degeneracies are unimportant.

### C. CHOOSING SIXTEEN MEASUREMENTS OUT OF THE THIRTY-TWO HETERODYNE DETECTIONS

Table S3 explicitly lists all 16 elements of  $\chi(T)$  which are extracted from the QPT protocol. As mentioned above, there are  $2^4 - 2^2 = 12$  independent real-valued parameters associated to the dynamics in the single exciton manifold, but we also keep track of four leakage errors  $\chi_{gg\alpha\alpha}(T)$ ,  $\chi_{gg\beta\beta}(T)$ , and  $\Re\{\chi_{gg\alpha\beta}(T)\}$  and  $\Im\{\chi_{gg\alpha\beta}(T)\}$ , yielding a total of sixteen parameters to extract. The terms associated with these transfers to the ground state are not listed, as they can be expressed in terms of the rest of the elements using Eq. (3) in the article. The sixteen experiments described in the article involve thirty-two heterodyne real valued measurements, twice as many as parameters to extract. Clearly, there must be a way to select only sixteen measurements out of the thirty-two. We now show that this reduction is feasible and has similar stability properties as the original set. It is important to emphasize that the thirty-two or sixteen required heterodyne detections are one-dimensional (1D) measurements, as the signals  $\langle [S_{PE}]_{\mathbf{e}_1, \mathbf{e}_2, \mathbf{e}_3, \mathbf{e}_4}^{\omega_1, \omega_2, \omega_3, \omega_4}(\tau, T, t) \rangle_{iso}$  stemming from a single pair of  $\tau, t$  values suffice for the purposes of performing a QPT.

We first make some observations which are easily generalizable. Altogether, the four terms  $\Re\{\langle P_{\mathbf{e}_1, \mathbf{e}_2, \mathbf{e}_3, \mathbf{e}_4}^{\alpha, \alpha, \alpha, \alpha}(\tau, T, t) \rangle_{iso}\}$ ,  $\Im\{\langle P_{\mathbf{e}_1, \mathbf{e}_2, \mathbf{e}_3, \mathbf{e}_4}^{\alpha, \alpha, \alpha, \alpha}(\tau, T, t) \rangle_{iso}\}$ ,  $\Re\{\langle P_{\mathbf{e}_1, \mathbf{e}_2, \mathbf{e}_3, \mathbf{e}_4}^{\alpha, \alpha, \beta, \beta}(\tau, T, t) \rangle_{iso}\}$ , and  $\Im\{\langle P_{\mathbf{e}_1, \mathbf{e}_2, \mathbf{e}_3, \mathbf{e}_4}^{\alpha, \alpha, \beta, \beta}(\tau, T, t) \rangle_{iso}\}$  contain information about the real valued population transfer terms  $\chi_{\alpha\alpha\alpha\alpha}(T)$  and  $\chi_{\beta\beta\alpha\alpha}(T)$ . Consider the case where  $\mathcal{G}_{gp}(\tau)\mathcal{G}_{ps}(t) \in \Re$  (for example, taking  $\tau$  and  $t$  to satisfy  $\omega_{gp}\tau = \omega_{ps}t = 2\pi$ ). Then, only  $\Re\{\langle P_{\mathbf{e}_1, \mathbf{e}_2, \mathbf{e}_3, \mathbf{e}_4}^{\alpha, \alpha, \alpha, \alpha}(\tau, T, t) \rangle_{iso}\}$  and  $\Re\{\langle P_{\mathbf{e}_1, \mathbf{e}_2, \mathbf{e}_3, \mathbf{e}_4}^{\alpha, \alpha, \beta, \beta}(\tau, T, t) \rangle_{iso}\}$  need to be monitored, as  $\Im\{\langle P_{\mathbf{e}_1, \mathbf{e}_2, \mathbf{e}_3, \mathbf{e}_4}^{\alpha, \alpha, \alpha, \alpha}(\tau, T, t) \rangle_{iso}\}$  and  $\Im\{\langle P_{\mathbf{e}_1, \mathbf{e}_2, \mathbf{e}_3, \mathbf{e}_4}^{\alpha, \alpha, \beta, \beta}(\tau, T, t) \rangle_{iso}\}$  will, in principle, vanish. Conversely, if  $\mathcal{G}_{gp}(\tau)\mathcal{G}_{ps}(t) \in \Im$  (say, by taking  $\omega_{gp}\tau = \frac{\pi}{2}$  and  $\omega_{ps}t = 2\pi$ ), only the imaginary parts need to be monitored. Finally, if  $\mathcal{G}_{gp}(\tau)\mathcal{G}_{ps}(t)$  has both real and complex parts of similar proportions, either the real or the imaginary parts suffice. Naturally, depending on the ratio between the magnitudes of the real and imaginary parts of  $\mathcal{G}_{gp}(\tau)\mathcal{G}_{ps}(t)$ , it will be numerically more favorable to measure the real or the imaginary parts of the signal.

Consider now the signals  $\Re\{\langle P_{z, z, z, z}^{\beta, \alpha, \beta, \alpha}(\tau, T, t) \rangle_{iso}\}$ ,  $\Im\{\langle P_{z, z, z, z}^{\beta, \alpha, \beta, \alpha}(\tau, T, t) \rangle_{iso}\}$ ,  $\Re\{\langle P_{z, z, z, z}^{\alpha, \beta, \alpha, \beta}(\tau, T, t) \rangle_{iso}\}$ , and  $\Im\{\langle P_{z, z, z, z}^{\alpha, \beta, \alpha, \beta}(\tau, T, t) \rangle_{iso}\}$ , which contain information about  $\Re\{\chi_{\alpha\beta\alpha\beta}(T)\}$  and  $\Im\{\chi_{\alpha\beta\alpha\beta}(T)\}$ . By proceeding as in the previous paragraph, it can be seen that either the first two or the last two are good enough to extract information about the latter two quantities.

The steps above can be repeated for the rest of the elements of  $\chi(T)$  in order to select sixteen out of the thirty-two measurements which yield the desired QPT. Table S7 presents an adaptation

of Table S3, where, in the first column, we show a possible set of experiments which yields QPT for the case of  $\mathcal{G}_{gp}(\tau)\mathcal{G}_{ps}(t)$  being purely real.

Table S7. A set of only sixteen measurements which yields  $\chi(T)$  for the case  $\mathcal{G}_{gp}(\tau)\mathcal{G}_{ps}(t) \in \mathbb{R}$

| From the data                                                                                                                                                                                                                                                                                                                                                                                                                                                                                                                                                                                                                                                                                                                                       | we can invert the elements                                  | which explicitly listed are                                                                                                                                                                                                                                                                                                                                                                                                                                                                                                                                                                                                                                                                                                                                     |
|-----------------------------------------------------------------------------------------------------------------------------------------------------------------------------------------------------------------------------------------------------------------------------------------------------------------------------------------------------------------------------------------------------------------------------------------------------------------------------------------------------------------------------------------------------------------------------------------------------------------------------------------------------------------------------------------------------------------------------------------------------|-------------------------------------------------------------|-----------------------------------------------------------------------------------------------------------------------------------------------------------------------------------------------------------------------------------------------------------------------------------------------------------------------------------------------------------------------------------------------------------------------------------------------------------------------------------------------------------------------------------------------------------------------------------------------------------------------------------------------------------------------------------------------------------------------------------------------------------------|
| $\left\{ \begin{array}{l} \Re\{\langle P_{z,z,z,z}^{\alpha,\alpha,\alpha,\alpha}(\tau, T, t) \rangle_{iso}\}, \\ \Re\{\langle P_{z,z,z,z}^{\alpha,\alpha,\alpha,\beta}(\tau, T, t) \rangle_{iso}\}, \\ \Im\{\langle P_{z,z,z,z}^{\alpha,\alpha,\alpha,\beta}(\tau, T, t) \rangle_{iso}\}, \\ \Re\{\langle P_{z,z,z,z}^{\alpha,\alpha,\beta,\beta}(\tau, T, t) \rangle_{iso}\} \end{array} \right\}$                                                                                                                                                                                                                                                                                                                                                 | $\{\chi_{ij\alpha\alpha}(T)\}$                              | $\left\{ \begin{array}{l} \chi_{\alpha\alpha\alpha\alpha}(T), \\ \chi_{\beta\beta\alpha\alpha}(T), \\ \Re\{\chi_{\alpha\beta\alpha\alpha}(T)\} = \Re\{\chi_{\beta\alpha\alpha\alpha}(T)\}, \\ \Im\{\chi_{\alpha\beta\alpha\alpha}(T)\} = -\Im\{\chi_{\beta\alpha\alpha\alpha}(T)\} \end{array} \right\}$                                                                                                                                                                                                                                                                                                                                                                                                                                                        |
| $\left\{ \begin{array}{l} \Re\{\langle P_{z,z,z,z}^{\beta,\beta,\alpha,\alpha}(\tau, T, t) \rangle_{iso}\}, \\ \Re\{\langle P_{z,z,z,z}^{\beta,\beta,\alpha,\beta}(\tau, T, t) \rangle_{iso}\}, \\ \Im\{\langle P_{z,z,z,z}^{\beta,\beta,\alpha,\beta}(\tau, T, t) \rangle_{iso}\}, \\ \Re\{\langle P_{z,z,z,z}^{\beta,\beta,\beta,\beta}(\tau, T, t) \rangle_{iso}\} \end{array} \right\}$                                                                                                                                                                                                                                                                                                                                                         | $\{\chi_{ij\beta\beta}(T)\}$                                | $\left\{ \begin{array}{l} \chi_{\alpha\alpha\beta\beta}(T), \\ \chi_{\beta\beta\beta\beta}(T), \\ \Re\{\chi_{\alpha\beta\beta\beta}(T)\} = \Re\{\chi_{\beta\alpha\beta\beta}(T)\}, \\ \Im\{\chi_{\alpha\beta\beta\beta}(T)\} = -\Im\{\chi_{\beta\alpha\beta\beta}(T)\} \end{array} \right\}$                                                                                                                                                                                                                                                                                                                                                                                                                                                                    |
| $\left\{ \begin{array}{l} \Re\{\langle P_{z,z,z,z}^{\beta,\alpha,\alpha,\alpha}(\tau, T, t) \rangle_{iso}\}, \\ \Im\{\langle P_{z,z,z,z}^{\beta,\alpha,\alpha,\alpha}(\tau, T, t) \rangle_{iso}\}, \\ \Re\{\langle P_{z,z,z,z}^{\beta,\alpha,\alpha,\beta}(\tau, T, t) \rangle_{iso}\}, \\ \Im\{\langle P_{z,z,z,z}^{\beta,\alpha,\alpha,\beta}(\tau, T, t) \rangle_{iso}\}, \\ \Re\{\langle P_{z,z,z,z}^{\beta,\alpha,\beta,\beta}(\tau, T, t) \rangle_{iso}\}, \\ \Im\{\langle P_{z,z,z,z}^{\beta,\alpha,\beta,\beta}(\tau, T, t) \rangle_{iso}\}, \\ \Re\{\langle P_{z,z,z,z}^{\beta,\alpha,\beta,\alpha}(\tau, T, t) \rangle_{iso}\}, \\ \Im\{\langle P_{z,z,z,z}^{\beta,\alpha,\beta,\alpha}(\tau, T, t) \rangle_{iso}\} \end{array} \right\}$ | $\{\chi_{ij\alpha\beta}(T) = (\chi_{ji\beta\alpha}(T))^*\}$ | $\left\{ \begin{array}{l} \Re\{\chi_{\alpha\alpha\alpha\beta}(T)\} = \Re\{\chi_{\alpha\alpha\beta\alpha}(T)\}, \\ \Im\{\chi_{\alpha\alpha\alpha\beta}(T)\} = -\Im\{\chi_{\alpha\alpha\beta\alpha}(T)\}, \\ \Re\{\chi_{\beta\beta\alpha\beta}(T)\} = \Re\{\chi_{\beta\beta\beta\alpha}(T)\}, \\ \Im\{\chi_{\beta\beta\alpha\beta}(T)\} = -\Im\{\chi_{\beta\beta\beta\alpha}(T)\}, \\ \Re\{\chi_{\alpha\beta\alpha\beta}(T)\} = \Re\{\chi_{\beta\alpha\beta\alpha}(T)\}, \\ \Im\{\chi_{\alpha\beta\alpha\beta}(T)\} = -\Im\{\chi_{\beta\alpha\beta\alpha}(T)\}, \\ \Re\{\chi_{\beta\alpha\alpha\beta}(T)\} = \Re\{\chi_{\alpha\beta\beta\alpha}(T)\}, \\ \Im\{\chi_{\beta\alpha\alpha\beta}(T)\} = -\Im\{\chi_{\alpha\beta\beta\alpha}(T)\} \end{array} \right\}$ |

The same calculation of Fig. S2 can be repeated for this setting, where  $\mathbb{M}^{qp}$  and  $P^{qp}(T)$  only contain the elements in the first column of Table S7. We do not show them because they have the same coarse appearance as the ones in Fig. S2. We make a numerical comparison between the matrices of  $\kappa$  values calculated in the previous subsection and the ones computed with the selective measurements of Table S7, where we round large values of  $\kappa$  down to be 100. We find relative differences in their 2-norms of 0.094, 0.12, 0.0023, and 0.0028 for the  $d_B/d_A = 1, 1.5, 10, 150$  cases, respectively, supporting the qualitative claim that the two protocols are similar in terms of stability.

## XII. SCALABILITY

The QPT protocol can be extended to general aggregates of  $d$  chromophores using a pulse toolbox of  $d$  different waveforms (the single exciton Hilbert space is size  $d$ ). Details will be provided in a future publication. For now, let us make a comparison between the number of

1D measurements required for a multichromophoric QPT and the effort involved in collecting a standard 2D-ES [26]. On the one hand, without keeping track of leakage errors, the number of required QPT 1D experiments is equal to the number of parameters to extract,  $d^4 - d^2$ . On the other hand, the number of grid points in a single 2D-ES, which we take as the effective number of experiments, is on the order of 7000 [21]. Therefore, within this crude measure, it is only for  $d > 10$  that a QPT becomes more costly than a single 2D-ES [27]. Clearly, the scalability of QPT as  $O(d^4)$  is not favorable asymptotically, although ideas associated with single shot setups [22] or compressed sensing [23, 24] could provide significant reductions in the required physical resources. However, this limit might not even be relevant at present. So far, the largest multichromophoric system for which spectral lineshapes can be resolved in a 2D-ES consists of the lowest lying states of the Light Harvesting Complex-II [25], corresponding to  $d = 14$ , giving  $14^4 - 14^2 = 38220$  1D experiments, which amounts to an effort of collecting about six 2D-ES.

- 
- [1] M.D. Choi. Completely positive linear maps on complex matrices. *Linear Algebra Appl.*, 10(3):285 – 290, 1975.
  - [2] E. C. G. Sudarshan, P. M. Mathews, and Jayaseetha Rau. Stochastic dynamics of quantum-mechanical systems. *Phys. Rev.*, 121(3):920–924, 1961.
  - [3] T. Mančal and G. R. Fleming. Probing electronic coupling in excitonically coupled heterodimer complexes by two-color three-pulse photon echoes. *J. Chem. Phys.*, 121:10556–10565, 2004.
  - [4] J. Yuen-Zhou and A. Aspuru-Guzik. Quantum process tomography of excitonic dimers from two-dimensional electronic spectroscopy. i. general theory and application to homodimers. *J. Chem. Phys.*, 134(13):134505, 2011.
  - [5] S. Mukamel. *Principles of Nonlinear Optical Spectroscopy*. Oxford University Press, 1995.
  - [6] D.P. Craig and T. Thirunamachandran. *Molecular quantum electrodynamics: An introduction to radiation molecule interactions*. Dover Publications, 1998.
  - [7] A. M. Kuah, K. Modi, C. A. Rodríguez-Rosario, and E. C. G. Sudarshan. How state preparation can affect a quantum experiment: Quantum process tomography for open systems. *Phys. Rev. A*, 76(4):042113, 2007.
  - [8] K. Modi and E. C. G. Sudarshan. Role of preparation in quantum process tomography. *Phys. Rev. A*, 81(5):052119, 2010.
  - [9] K. Modi. Non-Markovian memory in quantum process tomography and a preparation independent map. *ArXiv e-prints*, 2010.
  - [10] H. Lee, Y. C. Cheng, and G. R. Fleming. Coherence Dynamics in Photosynthesis: Protein

- Protection of Excitonic Coherence. *Science*, 316:1462–1465, 2007.
- [11] Hochstrasser R. M. Two-dimensional ir-spectroscopy: polarization anisotropy effects. *Chem. Phys.*, 266(2-3):273 – 284, 2001.
  - [12] G. S. Schlau-Cohen, T. R. Calhoun, N. S. Ginsberg, M. Ballottari, R. Bassi, and G. R. Fleming. Spectroscopic elucidation of uncoupled transition energies in the major photosynthetic light-harvesting complex, LHCII. *Proc. Natl. Acad. Sci. USA*, 107(30):13276–13281, 2010.
  - [13] D.B. Strasfeld, C.T. Middleton, and M.T. Zanni. Mode selectivity with polarization shaping in the mid-ir. *New J. Phys.*, 11(10):105046, 2009.
  - [14] M. Cho. *Two Dimensional Optical Spectroscopy*. CRC Press, 2009.
  - [15] D. M. Jonas. Two-dimensional femtosecond spectroscopy. *Ann. Rev. Phys. Chem.*, 54:425–463, 2003.
  - [16] S. M. Gallagher Faeder and D. M. Jonas. Two-dimensional electronic correlation and relaxation spectra: Theory and model calculations. *J. Phys. Chem. A*, 103(49):10489–10505, 1999.
  - [17] V. May and O. Kuhn. *Charge and Energy Transfer Dynamics in Molecular Systems*. Wiley-VCH, 2004.
  - [18] A. V. Pislakov, T. Mančal, and G. R. Fleming. Two-dimensional optical three-pulse photon echo spectroscopy. ii. signatures of coherent electronic motion and exciton population transfer in dimer two-dimensional spectra. *J. Chem. Phys.*, 124:234505, 2006.
  - [19] W. Cheney and D. Kincaid. *Numerical mathematics and computing*. Thomson-Brooks/Cole, sixth edition, 2008.
  - [20] R. A. Horn and Johnson C. R. *Matrix Analysis*. Cambridge University Press, 1990.
  - [21] M. T. Zanni, S. Gnanakaran, J. Stenger, and R. M. Hochstrasser. Heterodyned two-dimensional infrared spectroscopy of solvent-dependent conformations of acetylproline-nh2. *J. Phys. Chem. B*, 105(28):6520–6535, 2001.
  - [22] E. Harel, A. F. Fidler, and G. S. Engel. Real-time mapping of electronic structure with single-shot two-dimensional electronic spectroscopy. *Proc. Natl. Acad. Sci. USA*, 107(38):16444–16447, 2010.
  - [23] M. Mohseni, A. T. Rezakhani, and D. A. Lidar. Quantum-process tomography: Resource analysis of different strategies. *Phys. Rev. A*, 77:032322, 2008.
  - [24] A. Shabani, R. L. Kosut, M. Mohseni, H. Rabitz, M. A. Broome, M. P. Almeida, A. Fedrizzi, and A. G. White. Efficient measurement of quantum dynamics via compressive sensing. *Phys. Rev. Lett.*, 106(10):100401, 2011.
  - [25] T. R. Calhoun, N. S. Ginsberg, G. S. Schlau-Cohen, Y. C. Cheng, M. Ballottari, R. Bassi, and G. R. Fleming. Quantum coherence enabled determination of the energy landscape in light-harvesting complex ii. *J. Phys. Chem. B*, 113(51):16291–16295, 2009.

- [26] Contrasting the number of experiments in two different settings does not necessarily provide a fair estimate of the real effort, as an experimentalist might have built a machine that efficiently carries one type of measurement, but not the other. However, at least this provides an estimate of the resources involved in each situation.
- [27] As explained in point (b) above, QPT can also be performed with 2D-ES, but for large  $d$  values, precisely due to the reasons just outlined, the 1D setup is more convenient.
